# Supplementary material for: Quantifying uncertainty and dynamical changes in multi-species fishing mortality rates, catches and biomass by combining state-space and mechanistic multi-species models
Source: arXiv:2008.02765 ancillary file (2020-08-06)
Supplement: Supplementary file 1 [file Supplementary.pdf]

# Supplementary material

July 30, 2020

## S1 Model

Blanchard et al. (2014) developed a multi-species size spectrum model based on the equations of Hartvig et al. (2011) but with explicit representation of specific traits for the species and not just its asymptotic size. We describe the mizer model and the parameters used to in this study below.

### S1.1 Model description

The sized-based model is used to calculate the size- and trait-spectrum $N_i(m)$ which is the density of individuals such that $N_i(m)dm$ is the number of individuals of species $i$ in the size interval $[m, m + dm]$.

The process of reproduction, growth and mortality to the size spectrum of each trait group is achieved by the McKendrik-von Foerster conservation equation

$$\frac{\partial N_i(m)}{\partial t} + \frac{\partial \left(g_i(m) N_i(m)\right)}{\partial m} = -\mu_i(m) N_i(m), \tag{S1}$$

where $g_i(m)$ is the individual growth and $\mu_i(m)$ is the mortality. Both growth and mortality are determined by the availability of food from other species plus the background resource, $N_R(m)$, and predation by the other species, as explained below.

Equation S1 is supplemented by a boundary condition at $m_0$, the weight of an egg, so that the increase of the number of individuals, $g_i(m_0)N_i(m_0)$ is determined by

$$g_i(m_0)N_i(m_0) = R_i$$

where $R_i$ is the reproduction of the offspring by mature individuals in population $i$. Each species has its own preference in terms of the weights of prey that it will consume, expressed in terms of the ratio of weights between predator and prey. This is calculated by an unnormalised log-normal distribution

$$\phi_i(m_p/m) = \exp\left[-\frac{(\ln(\beta_i m_p/m))^2}{2\xi_i^2}\right].$$

### Predator-prey encounter

The food available for a predator of species $i$ of weight $m$ is

$$E_{a.i}(m) = \int \left( N_R(m_p) + \sum_{j=1}^{s} \Omega_{ij} N_j(m_p) \right) \phi_i(m_p/m) m dm_p \tag{S2}$$

where $\Omega_{ij}$ is the preference of species $i$ for species $j$ and $s$ is the number of species in the model. However the food encountered is dependent on the search rate $\gamma_i m^q$ and is determined by

$$E_{e.i} = \gamma_i m^q E_{a.i}.$$

### Consumption

The feeding level,

$$f_i(m) = \frac{E_{e.i}}{E_{e.i} + h_i m^n},$$

is a number between 0, where the individual gets no food, and 1, where the individual is fully satiated. $h$ is the maximum food intake and $n$ is the exponent for the maximum food intake.

### Somatic Growth

The energy available for growth and reproduction gained from consumption is

$$E_i(m) = \alpha f_i(m) h_i m^n - k_{s.i} m^p.$$

$\alpha$ is the efficiency parameter, $k_{s.i}$ is the energy required for standard metabolism and activity and $p$ is the exponent of standard metabolism. The energy used for reproduction is

$$\zeta_i(m) = \left[ 1 + \left( \frac{m}{m_{m.i}} \right)^{-u} \right]^{-1} \left( \frac{m}{W_i} \right)^{1-n},$$

where $m_{m.i}$ is the weight at maturation and $W_i$ is the asymptotic size of species $i$. The somatic growth is

$$g_i(m) = E_i(m)(1 - \zeta_i(m)).$$

### Reproduction

The total production of eggs is

$$R_{p.i} = \frac{\epsilon}{2m_0} \int N_i(m) E_i(m) \zeta_i(m) dm,$$

where $m_0$ is the egg weight, $\epsilon$ is the efficiency of reproduction and the 1/2 takes into account that only females reproduce (Hartvig et al., 2011; Scott et al., 2014).

### Recruitment

The recruitment is defined by

$$R_i = R_{max.i}\frac{R_{p.i}}{R_{p.i} + R_{max.i}}.$$

### Mortality

Mortality, $\mu_i(m)$, is the sum of the four types of mortality

$$\mu_i(m) = \mu_{p.i}(m) + \mu_{s.i}(m) + \mu_{b.i}(m) + \mu_{f.i}(m).$$

The predation mortality is defined as

$$\mu_{p.i}(m_p) = \sum_{j=1}^{s}\int \phi_j(m_p/m)(1 - f_j(m))\gamma_j m^q \Omega_{ji} N_j(m)dm$$

which is the sum over all of the species that have preyed on species $i$. This follows from the predation in equation S2. If $E_i(m) < 0$ then an individual doesn't receive enough energy to perform standard metabolism and activity and therefore has a starvation mortality, $\mu_{s.i}(m)$, such that

$$\mu_{s.i}(m) = \begin{cases} 0 & \text{if } E_i(m) > 0 \\ \frac{-E_i(m)}{\chi m} & \text{otherwise} \end{cases}$$

where $\chi$ is the fraction of energy reserves (Hartvig et al., 2011). The background mortality is

$$\mu_{b.i}(m) = \mu_0 W_i^z.$$

The fourth mortality is through fishing. The commercial catch of species $i$ is

$$\phi_i \int q_i(m)N_i(m)dm$$

where $\phi_i$ is the fishing rate and $q_i(m)$ is the size selectivity curve for species $i$. Similarly the surveyed catch of the $i$th species is

$$\phi_{sur} \int q_{sur,i}(m)N_i(m)dm$$

where $\phi_{sur}$ is the fishing rate of survey vessel and $q_{sur,i}$ is the catchability of the the $i$th species by the survey vessel.

### Resource dynamics

The background resource is

$$\frac{dN_R(m,t)}{dt} = r_0 m^{p-1}\left[\kappa m^{-\lambda} - N_R(m,t)\right] - \mu_p(m)N_R(m,t),$$

where $r_0 w^{p-1}$ is the population regeneration rate and the carrying capacity is $\kappa m^{-\lambda}$.

### Numerical solution

The model is solved by standard finite difference techniques. This was achieved by discretising both time and size. Here we used a time step of 0.25 years as in Spence et al. (2016). See Appendix G in Hartvig et al. (2011) and the mizer vignette for more details (Scott et al., 2014).

## S1.2 Parameters

Tables S1 and S2 give the value of $\Omega$, Table S3 gives the species specific parameters, which were fitted to survey data from ICES (2017), and Table S4 gives other fixed parameter values, which are the same as those in Blanchard et al. (2014).

## S1.3 Fishing mortality

The model enables the fishing mortality to be varied overtime. The commercial fishing had a knife edge selectivity,

$$q_i(m) = \begin{cases} 1 & \text{if } m \geq w_{m.i} \\ 0 & \text{otherwise,} \end{cases}$$

and the survey selectivity was calculated from Walker et al. (2017). The selectivity of the commercial and survey gears are shown in Figures S1 and S2.

The commercial catches in the $t$th year, $\boldsymbol{c}(M_t)$, is a vector of length 17 where the $i$th element was

$$c(M_t)_i = \phi_{t,i} \int_{t-1}^{t} \int q_i(m) N_i(m, \tau) dm d\tau. \tag{S3}$$

The survey catches in the $t$th year, $\boldsymbol{s}(M_t)$, is a vector of length 17 where the $i$th element was

$$s(M_t)_i = \phi_{t,sur} \int_{t-1}^{t} \int q_{sur,i}(m) N_i(m, \tau) dm d\tau. \tag{S4}$$

The survey effort, $\phi_{t,sur}$, is shown in Figure S3.

# S2 Markov Chain Monte Carlo

We sampled from the posterior distribution using a Markov Chain Monte Carlo algorithm. In this section we describe some of the specific moves we used when running the algorithm.

Table S1: The interaction matrix $\Omega$.

| | Herring | Sprat | Cod | Haddock | Whiting | Blue whiting | Norway Pout | Poor Cod | European Hake |
|---|---|---|---|---|---|---|---|---|---|
| Herring | 1 | 0.820 | 0.615 | 0.577 | 0.697 | 0.482 | 0.656 | 0.552 | 0.536 |
| Sprat | 0.820 | 1 | 0.580 | 0.584 | 0.678 | 0.473 | 0.627 | 0.562 | 0.541 |
| Cod | 0.615 | 0.580 | 1 | 0.726 | 0.706 | 0.678 | 0.666 | 0.718 | 0.731 |
| Haddock | 0.577 | 0.584 | 0.726 | 1 | 0.788 | 0.835 | 0.670 | 0.848 | 0.889 |
| Whiting | 0.697 | 0.678 | 0.706 | 0.788 | 1 | 0.694 | 0.678 | 0.796 | 0.782 |
| Blue whiting | 0.482 | 0.473 | 0.678 | 0.835 | 0.694 | 1 | 0.587 | 0.774 | 0.890 |
| Norway Pout | 0.656 | 0.627 | 0.666 | 0.670 | 0.678 | 0.587 | 1 | 0.642 | 0.636 |
| Poor Cod | 0.552 | 0.562 | 0.718 | 0.848 | 0.796 | 0.774 | 0.642 | 1 | 0.864 |
| European Hake | 0.536 | 0.541 | 0.731 | 0.889 | 0.782 | 0.890 | 0.636 | 0.864 | 1 |
| Monkfish | 0.560 | 0.562 | 0.721 | 0.767 | 0.693 | 0.769 | 0.612 | 0.749 | 0.797 |
| Horse Mackerel | 0.520 | 0.529 | 0.669 | 0.833 | 0.770 | 0.804 | 0.590 | 0.929 | 0.863 |
| Mackerel | 0.605 | 0.569 | 0.661 | 0.825 | 0.831 | 0.793 | 0.636 | 0.808 | 0.857 |
| Common Dab | 0.832 | 0.801 | 0.628 | 0.616 | 0.738 | 0.514 | 0.656 | 0.588 | 0.569 |
| Plaice | 0.659 | 0.606 | 0.575 | 0.533 | 0.592 | 0.456 | 0.676 | 0.495 | 0.486 |
| Megrim | 0.410 | 0.416 | 0.638 | 0.792 | 0.639 | 0.808 | 0.601 | 0.725 | 0.826 |
| Sole | 0.435 | 0.408 | 0.374 | 0.311 | 0.354 | 0.301 | 0.358 | 0.280 | 0.305 |
| Boarfish | 0.395 | 0.398 | 0.611 | 0.747 | 0.609 | 0.754 | 0.526 | 0.719 | 0.800 |

Table S2: The interaction matrix $\Omega$.

| | Monkfish | Horse Mackerel | Mackerel | Common Dab | Plaice | Megrim | Sole | Boarfish |
|---|---|---|---|---|---|---|---|---|
| Herring | 0.560 | 0.520 | 0.605 | 0.832 | 0.659 | 0.410 | 0.435 | 0.395 |
| Sprat | 0.562 | 0.529 | 0.569 | 0.801 | 0.606 | 0.416 | 0.408 | 0.398 |
| Cod | 0.721 | 0.669 | 0.661 | 0.628 | 0.575 | 0.638 | 0.374 | 0.611 |
| Haddock | 0.767 | 0.833 | 0.825 | 0.616 | 0.533 | 0.792 | 0.311 | 0.747 |
| Whiting | 0.693 | 0.770 | 0.831 | 0.738 | 0.592 | 0.639 | 0.354 | 0.609 |
| Blue whiting | 0.769 | 0.804 | 0.793 | 0.514 | 0.456 | 0.808 | 0.301 | 0.754 |
| Norway Pout | 0.612 | 0.590 | 0.636 | 0.656 | 0.676 | 0.601 | 0.358 | 0.526 |
| Poor Cod | 0.749 | 0.929 | 0.808 | 0.588 | 0.495 | 0.725 | 0.280 | 0.719 |
| European Hake | 0.797 | 0.863 | 0.857 | 0.569 | 0.486 | 0.826 | 0.305 | 0.800 |
| Monkfish | 1 | 0.723 | 0.722 | 0.584 | 0.520 | 0.699 | 0.338 | 0.685 |
| Horse Mackerel | 0.723 | 1 | 0.832 | 0.549 | 0.451 | 0.742 | 0.273 | 0.739 |
| Mackerel | 0.722 | 0.832 | 1 | 0.644 | 0.534 | 0.732 | 0.324 | 0.723 |
| Common Dab | 0.584 | 0.549 | 0.644 | 1 | 0.631 | 0.449 | 0.409 | 0.432 |
| Plaice | 0.520 | 0.451 | 0.534 | 0.631 | 1 | 0.425 | 0.421 | 0.345 |
| Megrim | 0.699 | 0.742 | 0.732 | 0.449 | 0.425 | 1 | 0.242 | 0.810 |
| Sole | 0.338 | 0.273 | 0.324 | 0.409 | 0.421 | 0.242 | 1 | 0.218 |
| Boarfish | 0.685 | 0.739 | 0.723 | 0.432 | 0.345 | 0.810 | 0.218 | 1 |

Table S3: The species specific parameters. $m_m$ and $W$ is the weight of maturity and asymptotic weight respectively measured in grams. $k_{s.i}$ is the empirical von Bertalanffy growth rate ($\mathrm{yr}^{-1}$), $\beta_i$ is the preferred predator-prey mass ratio and $\xi$ is the variance of this on the log-scale. $\ln\gamma$ is the volumetric search rate ($\mathrm{g}^{-q}\mathrm{yr}^{-1}$) and $h$ is the standard metabolism ($\mathrm{g}^{1-n}\mathrm{yr}^{-1}$).

| $i$ | Species | $m_m$ | $W$ | $k_s$ | $\beta$ | $\xi$ | $\ln\gamma$ | $h$ |
|---|---|---|---|---|---|---|---|---|
| 1 | Herring | 101.516 | 224.601 | 0.550 | 280,540 | 3.200 | −25.114 | 27.841 |
| 2 | Sprat | 6.182 | 22.717 | 0.645 | 51,076 | 0.800 | −24.019 | 15.220 |
| 3 | Cod | 1,124.216 | 13,983.910 | 0.250 | 66 | 1.300 | −22.434 | 50.152 |
| 4 | Haddock | 208.232 | 1,064.834 | 0.349 | 558 | 2.100 | −23.746 | 29.728 |
| 5 | Whiting | 67.456 | 709.147 | 0.437 | 22 | 1.500 | −22.870 | 32.510 |
| 6 | Blue whiting | 20.530 | 182.054 | 0.498 | 100 | 1.500 | −23.395 | 23.528 |
| 7 | Norway Pout | 18.622 | 79.424 | 0.551 | 21.500 | 1.500 | −23.366 | 19.728 |
| 8 | Poor Cod | 27.913 | 84.800 | 0.500 | 110 | 1.400 | −23.587 | 18.306 |
| 9 | European Hake | 281.270 | 9,752.278 | 0.211 | 11 | 1.100 | −22.312 | 37.626 |
| 10 | Monkfish | 543.469 | 9,030.276 | 0.164 | 16 | 1.200 | −22.729 | 28.482 |
| 11 | Horse Mackerel | 34.346 | 216.016 | 0.497 | 225 | 1.500 | −23.448 | 24.854 |
| 12 | Mackerel | 161.384 | 498.769 | 0.369 | 100 | 1.500 | −23.359 | 24.391 |
| 13 | Common Dab | 9.320 | 358.846 | 0.245 | 191 | 1.900 | −24.213 | 14.509 |
| 14 | Plaice | 117.919 | 466.706 | 0.360 | 113 | 1.600 | −23.490 | 23.251 |
| 15 | Megrim | 127.695 | 1,809.546 | 0.118 | 85 | 1.400 | −23.978 | 11.957 |
| 16 | Sole | 55.101 | 473.613 | 0.407 | 381 | 1.900 | −23.704 | 26.459 |
| 17 | Boarfish | 14.280 | 52.980 | 0.256 | 85,000 | 2 | −25.676 | 8.001 |

| Par | Description | Value | Units |
|---|---|---|---|
| $\alpha$ | Assimilation efficiency | 0.6 | |
| $\epsilon$ | Reproductive efficiency | 1 | |
| $m_0$ | Egg weight | 0.001 | g |
| $n$ | Exponent of max. consumption | 2/3 | |
| $q$ | Exponent of search volume | 0.8 | |
| $p$ | Exponent of standard metabolism | 0.7 | |
| $\mu_0$ | Pre-factor for background mortality | 0.6 | $\text{yr}^{-1}$ |
| $z$ | Exponent of background mortality | -1/3 | $\text{g}^{1-n}\text{yr}^{-1}$ |
| $\lambda$ | Exponent of resource spectrum | $2 + q + n$ | |
| $r_0$ | Productivity of resource spectrum | 10 | $\text{g}^{1-n}\text{yr}^{-1}$ |
| $s$ | The number of species in the model | 12 | |

Table S4: Other parameters fixed values.

### S2.1 Parallel MCMC

When the likelihood, $l(\theta|\boldsymbol{x})$, is slow to calculate, the Metropolis-Hastings algorithm could be sped up by a method suggested by Cui et al. (2011). At each time step the MCMC chain proposes $n$ points to move to. At each of these points the likelihood is calculated and then the first of the point is considered. If it is rejected the second is considered, then the third and so on until either one of the points has been accepted or all of the points have been rejected. It is essentially saying that conditional on the current point, a proposed point being rejected and the next proposed point are independent of one another and therefore can be run in parallel. This algorithm speeds up the the Metropolis-Hastings algorithm up as a number of likelihoods are estimated in parallel. This is summed up in Algorithm S1.

### S2.2 Calderhead's Parallel MCMC

We describe Calderhead's parallel MCMC algorithm in algorithm S2 (Calderhead, 2014). In this algorithm several new points are proposed in parallel and then a finite state Markov Chain is used to move between the proposed points.

## S3 Proofs

### S3.1 Marginal-delayed-acceptance MCMC

The Marginal-delayed-acceptance MCMC (MDA-MCMC) algorithm is shown in Algorithm S3. To prove that this samples from the correct posterior distribution we need to satisfy detailed-balance.

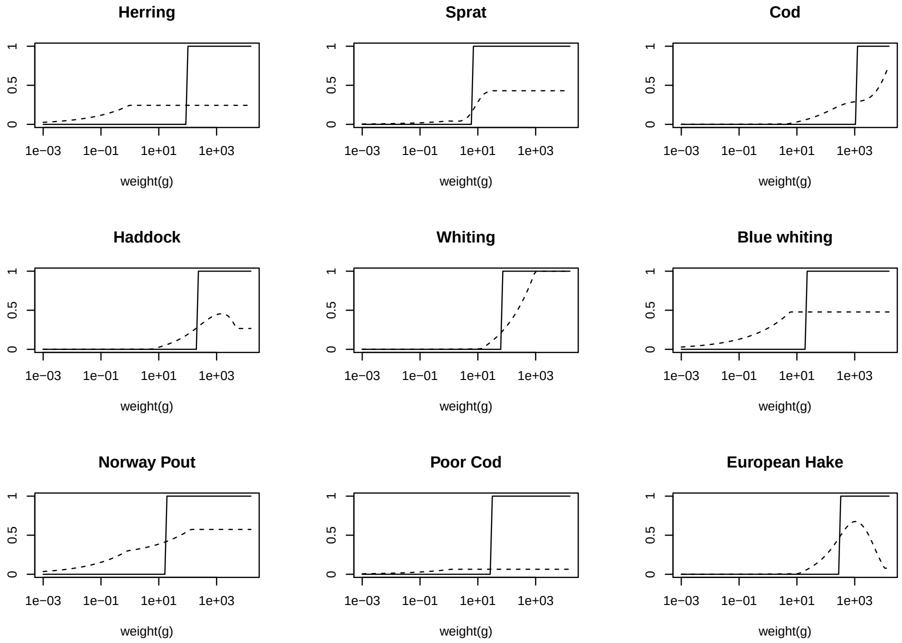


Figure S1: The gear selectivity for the first 9 species.

Let the uncertain parameters $\boldsymbol{\theta}$, with target distribution $\pi(\boldsymbol{\theta})$, be divided into three sets $\{\boldsymbol{\omega}\}$, $\{\boldsymbol{\mu}\}$, $\{\boldsymbol{\lambda}\}$, with likelihood evaluations $\pi_{\boldsymbol{\omega}}(\boldsymbol{\omega},\boldsymbol{\mu},\boldsymbol{\lambda})$, $\pi_{\boldsymbol{\mu}}(\boldsymbol{\omega},\boldsymbol{\mu},\boldsymbol{\lambda})$ and $\pi_{\boldsymbol{\lambda}}(\boldsymbol{\omega},\boldsymbol{\mu},\boldsymbol{\lambda})$ respectively. Without loss of generality let's presume that in a single step the Markov Chain moves $\{\boldsymbol{\omega},\boldsymbol{\mu},\boldsymbol{\lambda}\} \to \{\boldsymbol{\omega},\boldsymbol{\mu}',\boldsymbol{\lambda}'\}$, i.e. we accept $\boldsymbol{\mu}'$ and $\boldsymbol{\lambda}'$ but reject $\boldsymbol{\omega}'$. Now

$$\begin{aligned}\pi(\boldsymbol{\omega},\boldsymbol{\mu},\boldsymbol{\lambda})P(\{\boldsymbol{\omega},\boldsymbol{\mu},\boldsymbol{\lambda}\} \to \{\boldsymbol{\omega},\boldsymbol{\mu}',\boldsymbol{\lambda}'\}) \quad = \quad & \pi(\boldsymbol{\omega},\boldsymbol{\mu},\boldsymbol{\lambda})f(\boldsymbol{\omega}'|\boldsymbol{\omega})\left(1-\frac{\pi_{\boldsymbol{\omega}}(\boldsymbol{\omega}',\boldsymbol{\mu},\boldsymbol{\lambda})}{\pi_{\boldsymbol{\omega}}(\boldsymbol{\omega},\boldsymbol{\mu},\boldsymbol{\lambda})}\right)\\ & \times f(\boldsymbol{\mu}'|\boldsymbol{\mu})\left(1\wedge\frac{\pi_{\boldsymbol{\mu}}(\boldsymbol{\omega},\boldsymbol{\mu}',\boldsymbol{\lambda})}{\pi_{\boldsymbol{\mu}}(\boldsymbol{\omega},\boldsymbol{\mu},\boldsymbol{\lambda})}\right)\\ & \times f(\boldsymbol{\lambda}'|\boldsymbol{\lambda})\left(1\wedge\frac{\pi_{\boldsymbol{\lambda}}(\boldsymbol{\omega},\boldsymbol{\mu},\boldsymbol{\lambda}')}{\pi_{\boldsymbol{\lambda}}(\boldsymbol{\omega},\boldsymbol{\mu},\boldsymbol{\lambda})}\right)\\ & \times\alpha(\{\boldsymbol{\omega},\boldsymbol{\mu}',\boldsymbol{\lambda}'\},\{\boldsymbol{\omega},\boldsymbol{\mu},\boldsymbol{\lambda}\}), \qquad \text{(S5)}\end{aligned}$$

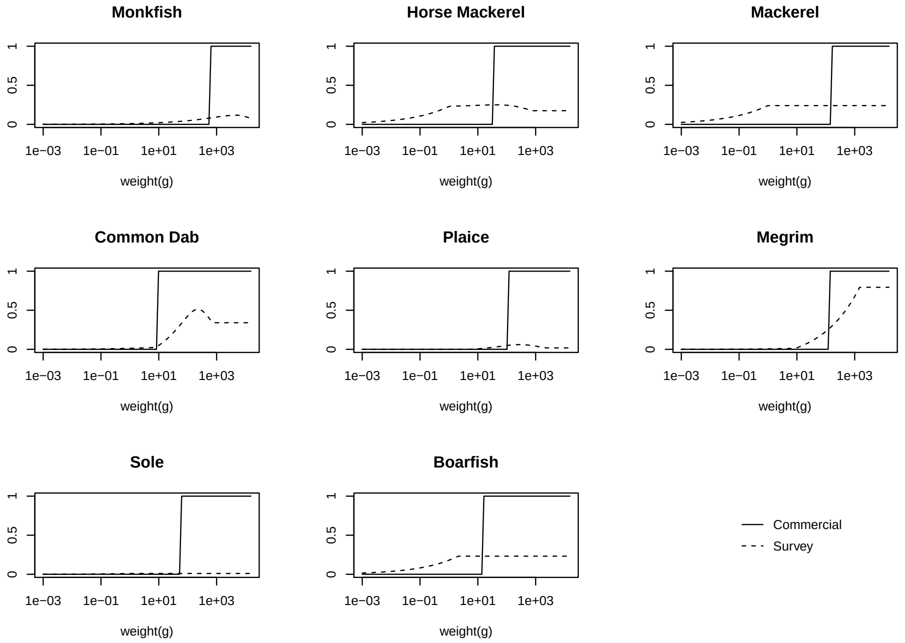


Figure S2: The gear selectivity for the last 8 species.

where $\wedge$ is the minimum, i.e. $a \wedge b = \min(a, b)$, with

$$\alpha(\{\boldsymbol{\omega}, \boldsymbol{\mu}', \boldsymbol{\lambda}'\}, \{\boldsymbol{\omega}, \boldsymbol{\mu}, \boldsymbol{\lambda}\}) = \left(1 \wedge \frac{\pi(\boldsymbol{\omega}, \boldsymbol{\mu}', \boldsymbol{\lambda}')}{\pi(\boldsymbol{\omega}, \boldsymbol{\mu}, \boldsymbol{\lambda})} \times \frac{\left(1 - \frac{\pi_{\boldsymbol{\omega}}(\boldsymbol{\omega}', \boldsymbol{\mu}', \boldsymbol{\lambda}')}{\pi_{\boldsymbol{\omega}}(\boldsymbol{\omega}, \boldsymbol{\mu}', \boldsymbol{\lambda}')}\right)}{\left(1 - \frac{\pi_{\boldsymbol{\omega}}(\boldsymbol{\omega}', \boldsymbol{\mu}, \boldsymbol{\lambda})}{\pi_{\boldsymbol{\omega}}(\boldsymbol{\omega}, \boldsymbol{\mu}, \boldsymbol{\lambda})}\right)} \times \frac{f(\boldsymbol{\mu}|\boldsymbol{\mu}')\left(1 \wedge \frac{\pi_{\boldsymbol{\mu}}(\boldsymbol{\omega}, \boldsymbol{\mu}, \boldsymbol{\lambda}')}{\pi_{\boldsymbol{\mu}}(\boldsymbol{\omega}, \boldsymbol{\mu}', \boldsymbol{\lambda}')}\right)}{f(\boldsymbol{\mu}'|\boldsymbol{\mu})\left(1 \wedge \frac{\pi_{\boldsymbol{\mu}}(\boldsymbol{\omega}, \boldsymbol{\mu}', \boldsymbol{\lambda})}{\pi_{\boldsymbol{\mu}}(\boldsymbol{\omega}, \boldsymbol{\mu}, \boldsymbol{\lambda})}\right)} \times \frac{f(\boldsymbol{\lambda}|\boldsymbol{\lambda}')\left(1 \wedge \frac{\pi_{\boldsymbol{\lambda}}(\boldsymbol{\omega}, \boldsymbol{\mu}', \boldsymbol{\lambda})}{\pi_{\boldsymbol{\lambda}}(\boldsymbol{\omega}, \boldsymbol{\mu}', \boldsymbol{\lambda}')}\right)}{f(\boldsymbol{\lambda}'|\boldsymbol{\lambda})\left(1 \wedge \frac{\pi_{\boldsymbol{\lambda}}(\boldsymbol{\omega}, \boldsymbol{\mu}, \boldsymbol{\lambda}')}{\pi_{\boldsymbol{\lambda}}(\boldsymbol{\omega}, \boldsymbol{\mu}, \boldsymbol{\lambda})}\right)}\right).$$

Without loss of generality, let $\alpha(\{\boldsymbol{\omega}, \boldsymbol{\mu}', \boldsymbol{\lambda}'\}, \{\boldsymbol{\omega}, \boldsymbol{\mu}, \boldsymbol{\lambda}\}) < 1$ then equation S5

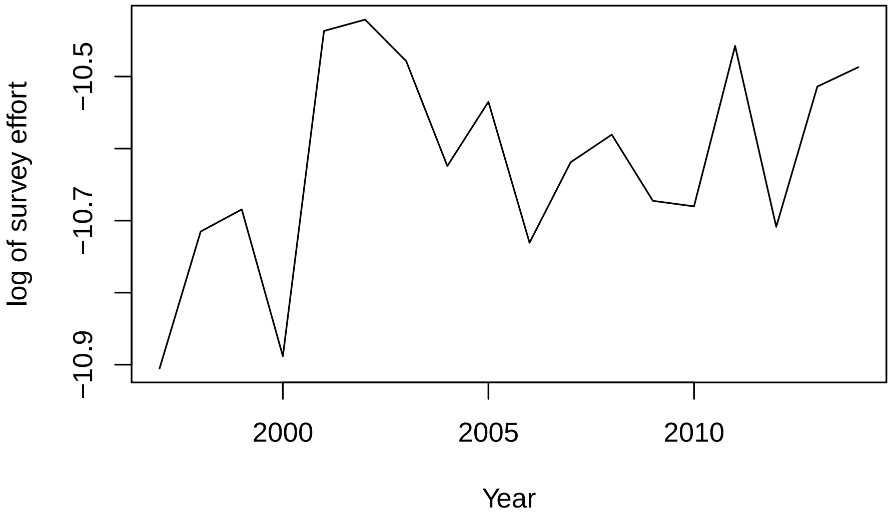


Figure S3: The effort for the survey vessel.

becomes

$$\begin{aligned} & \pi(\boldsymbol{\omega},\boldsymbol{\mu},\boldsymbol{\lambda}) f(\boldsymbol{\omega}'|\boldsymbol{\omega}) \left(1 - \frac{\pi_{\boldsymbol{\omega}}(\boldsymbol{\omega}',\boldsymbol{\mu}',\boldsymbol{\lambda}')}{\pi_{\boldsymbol{\omega}}(\boldsymbol{\omega},\boldsymbol{\mu}',\boldsymbol{\lambda}')}\right) \\ & \times f(\boldsymbol{\mu}|\boldsymbol{\mu}') \left(1 \wedge \frac{\pi_{\boldsymbol{\mu}}(\boldsymbol{\omega},\boldsymbol{\mu},\boldsymbol{\lambda}')}{\pi_{\boldsymbol{\mu}}(\boldsymbol{\omega},\boldsymbol{\mu}',\boldsymbol{\lambda}')}\right) \\ & \times f(\boldsymbol{\lambda}|\boldsymbol{\lambda}') \left(1 \wedge \frac{\pi_{\boldsymbol{\lambda}}(\boldsymbol{\omega},\boldsymbol{\mu}',\boldsymbol{\lambda})}{\pi_{\boldsymbol{\lambda}}(\boldsymbol{\omega},\boldsymbol{\mu}',\boldsymbol{\lambda}')}\right) \\ & \alpha(\{\boldsymbol{\omega},\boldsymbol{\mu},\boldsymbol{\lambda}\},\{\boldsymbol{\omega},\boldsymbol{\mu}',\boldsymbol{\lambda}'\}) \\ = \; & \pi(\boldsymbol{\omega},\boldsymbol{\mu}',\boldsymbol{\lambda}') P(\{\boldsymbol{\omega},\boldsymbol{\mu}',\boldsymbol{\lambda}'\} \to \{\boldsymbol{\omega},\boldsymbol{\mu},\boldsymbol{\lambda}\}) \end{aligned}$$

as $\alpha(\{\boldsymbol{\omega},\boldsymbol{\mu},\boldsymbol{\lambda}\},\{\boldsymbol{\omega},\boldsymbol{\mu}',\boldsymbol{\lambda}'\}) = 1$. Hence we have satisfied detailed balance.

### S3.2 Particle-delayed-acceptance MCMC

The Particle-delayed-acceptance MCMC (PDA-MCMC) algorithm is shown in Algorithm S4. To prove that this samples from the correct posterior distribution we need to satisfy detailed-balance.

For the stationary distribution $\pi(\phi)$ then

$$\pi(\phi)P(\phi \to \phi'') = \pi(\phi) f_{all}(\phi'',\phi'|\phi)\alpha_{all}(\phi,\phi'') \tag{S6}$$

**Algorithm S1** The parallel Metropolis-Hastings algorithm after $t$ iterations for target distribution $\pi(\boldsymbol{\theta})$. Given current value $\boldsymbol{\theta}_t$ and proposal distribution $f(\cdot|\boldsymbol{\theta})$. We define $\wedge$ to be the minimum, i.e. $a \wedge b = \min(a, b)$.

Generate $M$ candidate points $\boldsymbol{\theta}'_i \sim f(\cdot|\boldsymbol{\theta}_t)$
$j \leftarrow 0$
**while** $j < M$ or there is an accepted point **do**
    $j \leftarrow j + 1$
    $\alpha \leftarrow 1 \wedge \frac{\pi(\boldsymbol{\theta}')f(\boldsymbol{\theta}_t|\boldsymbol{\theta}'_j)}{\pi(\boldsymbol{\theta}_t)f(\boldsymbol{\theta}'_j|\boldsymbol{\theta}_t)}$
    Sample $u \sim \mathrm{U}(0, 1)$
    **if** $u < \alpha$ **then**
        $\boldsymbol{\theta}_{t+1} \leftarrow \boldsymbol{\theta}'$
    **else**
        $\boldsymbol{\theta}_{t+1} \leftarrow \boldsymbol{\theta}_t$
        $t \leftarrow t + 1$
    **end if**
**end while**

where $f_{all}(\phi'', \phi'|\phi)$ is the proposal of all $\phi''$ and $\phi'$ and is

$$\prod_{\{t:\phi_t \neq \phi''_t\}} \alpha(\phi_t, \phi'_t) \times \prod_{\{t:\phi_t = \phi''_t\}} 1 - \alpha(\phi_t, \phi'_t) \times \prod_{t=1}^{T} f(\phi'_t|\phi), \tag{S7}$$

and

$$\begin{aligned}\alpha_{all}(\phi, \phi'') = 1 \wedge \quad & \frac{\pi(\phi'')}{\pi(\phi)} \\ \times & \prod_{\{t:\phi_t \neq \phi''_t\}} \frac{f(\phi_t|\phi'_t)}{f(\phi'_t|\phi_t)} \times \frac{1 \wedge \frac{k_t(Q_t)}{k_t(Q'_t)}}{\alpha(\phi_t, \phi'_t)} \\ \times & \prod_{\{t:\phi_t = \phi''_t\}} \frac{1 - 1 \wedge \frac{k_t(Q'_t)}{k_t(Q_t)}}{1 - \alpha(\phi_t, \phi'_t)}\end{aligned}$$

which can be re-written as

$$\alpha_{all}(\phi, \phi'') = 1 \ \wedge \left( \frac{\pi(\phi'')}{\pi(\phi)} \times \frac{1}{f_{all}(\phi'', \phi'|\phi)} \times f_{all}(\phi, \phi'|\phi''). \right),$$

as

$$\begin{aligned} f_{all}(\phi, \phi'|\phi'') \quad = \quad & \prod_{\{t:\phi_t \neq \phi''_t\}} \frac{f(\phi_t|\phi'_t)}{f(\phi'_t|\phi_t)} \times 1 \wedge \frac{k_t(Q_t)}{k_t(Q'_t)} \\ & \times \prod_{\{t:\phi_t = \phi''_t\}} 1 - 1 \wedge \frac{k_t(Q'_t)}{k_t(Q_t)}. \end{aligned}$$

**Algorithm S2** $M$ iterations of Calderhead's parallel MCMC for target distribution $\pi(\boldsymbol{\theta})$. Given current value $\boldsymbol{\theta}$ and proposal distribution $f(\cdot|\boldsymbol{\theta})$.

$\boldsymbol{\theta}'_1 \leftarrow \boldsymbol{\theta}$
$\boldsymbol{z} \sim f(\cdot|\boldsymbol{\theta}_1)$
**for** $i = 2 : N$ **do**
  $\boldsymbol{\theta}'_i \sim f(\cdot|\boldsymbol{z})$
**end for**
**for** $i = 1 : N$ **do**
  $p_i \leftarrow \pi(\boldsymbol{\theta}'_i)K(i, -i)$ where

$$K(i, -i) = \frac{f(\boldsymbol{z}|\boldsymbol{\theta}'_i)\sum_{j\neq i} f(\boldsymbol{\theta}'_j|\boldsymbol{z})}{f(\boldsymbol{\theta}'_i|\boldsymbol{z})\sum_{j\neq i} f(\boldsymbol{z}|\boldsymbol{\theta}'_j)}$$

**end for**
The next $M$ iterations of the algorithm are sampled from $\boldsymbol{\theta}'_{1:N}$ with probabilities $p_{1:N}$

Without loss of generality let

$$\alpha_{all}(\phi, \phi'') = \left(\frac{\pi(\phi'')}{\pi(\phi)} \times \frac{1}{f_{all}(\phi'', \phi'|\phi)} \times f_{all}(\phi, \phi'|\phi'')\right) < 1,$$

then $\alpha_{all}(\phi'', \phi) = 1$ and equation S6 becomes

$$\begin{aligned} \pi(\phi)P(\phi \to \phi'') &= \pi(\phi) f_{all}(\phi'', \phi'|\phi)\frac{\pi(\phi'')}{\pi(\phi)} \\ &\quad \times \frac{1}{f_{all}(\phi'', \phi'|\phi)} \times f_{all}(\phi, \phi'|\phi'')\alpha_{all}(\phi'', \phi) \\ &= \pi(\phi'') f_{all}(\phi, \phi'|\phi'')\alpha_{all}(\phi'', \phi) \\ &= \pi(\phi'')P(\phi'' \to \phi) \end{aligned}$$

Hence we have satisfied detailed balance.

# S4 Results

## S4.1 History matching

We generated 500 combinations of the 35 static model parameters, $\boldsymbol{\theta}$ and the first year's fishing rates $\phi_{1:17,1}$ using Sobol' sequences (Sobol', 1967) from their respective prior distributions. We compared the simulated commercial catches in the first year to the observed catches. Figure S4 shows the modelled commercial landing for the first year, with the grey line being the observation, for different values of $\ln \kappa$. From this figure it is clear that $\ln \kappa > 20$. Figures S5 and S6 show the modelled commercial catches for

**Algorithm S3** An iteration of the marginal-delayed-acceptance MCMC algorithm (MDA-MCMC). The current parameters $\boldsymbol{\theta}$, are divided into $N+1$ disjoint sets with the $i$th set having likelihood evaluations $\pi_i(\boldsymbol{\theta})$ and proposal distribution $f_i(\cdot|\boldsymbol{\theta}_i)$. The full target distribution is $\pi(\boldsymbol{\theta})$. We define $\wedge$ to be the minimum, i.e. $a \wedge b = \min(a, b)$.

$\boldsymbol{\theta}'' \leftarrow \boldsymbol{\theta}$
**for** $i$ in $1 : N$ **do**
  $\boldsymbol{\theta}'_{\boldsymbol{i}} \sim f_i(\cdot|\boldsymbol{\theta}_i)$
  $\boldsymbol{\theta}''_{\boldsymbol{i}} \leftarrow \boldsymbol{\theta}'_{\boldsymbol{i}}$ with probability

$$\alpha_i(\boldsymbol{\theta}, \boldsymbol{\theta}'_i) = 1 \wedge \frac{\pi_i(\boldsymbol{\theta}'_i, \boldsymbol{\theta}_{-i})}{\pi_i(\boldsymbol{\theta})}$$

**end for**
$\boldsymbol{\theta} \leftarrow \boldsymbol{\theta}''$ with probability

$$\begin{aligned} 1 \wedge \quad & \frac{\pi(\boldsymbol{\theta}'')}{\pi(\boldsymbol{\theta})} \\ \times \quad & \prod_{\{i:\boldsymbol{\theta}''_i \neq \boldsymbol{\theta}_i\}} \frac{f_i(\boldsymbol{\theta}_i|\boldsymbol{\theta}'_i)}{f_i(\boldsymbol{\theta}'_i|\boldsymbol{\theta}_i)} \times \frac{\alpha_i(\boldsymbol{\theta}'', \boldsymbol{\theta}_i)}{\alpha_i(\boldsymbol{\theta}, \boldsymbol{\theta}'_i)} \\ \times \quad & \prod_{\{i:\boldsymbol{\theta}''_i = \boldsymbol{\theta}_i\}} \frac{1 - \alpha_i(\boldsymbol{\theta}'', \boldsymbol{\theta}'_i)}{1 - \alpha_i(\boldsymbol{\theta}, \boldsymbol{\theta}'_i)} \end{aligned}$$

**Algorithm S4** An iteration of the particle-delayed-acceptance MCMC algorithm (PDA-MCMC). Let $M_t = h(M_{t-1}, \phi_t, \boldsymbol{\theta})$ be the model run up until time $t$, with $M_0$ being its initial state and $k_t(M_t)$ be a likelihood evaluation of this model. The model is run up to time $T$. The static parameters are $\boldsymbol{\theta}$, the current fishing rates are $\phi$ and $f(\cdot|\phi_t)$ is the proposal distribution. The full target distribution is $\pi(\phi)$. We define $\wedge$ to be the minimum, i.e. $a \wedge b = \min(a, b)$.

---

$Q_0 \leftarrow M_0$, $\phi'' \leftarrow \phi$
**for** $t$ in $1 : T$ **do**
  $\phi'_t \sim f(\cdot|\phi_t)$
  $M'_t \leftarrow h(M_{t-1}, \phi'_t, \boldsymbol{\theta})$ and $M_t \leftarrow h(M_{t-1}, \phi_t, \boldsymbol{\theta})$
  $Q'_t \leftarrow h(Q_{t-1}, \phi'_t, \boldsymbol{\theta})$ and $Q_t \leftarrow h(Q_{t-1}, \phi_t, \boldsymbol{\theta})$

  $\phi''_t \leftarrow \phi'_t$ and $M_t \leftarrow M'_t$ with probability

$$\alpha_t(\phi_t, \phi'_t) = 1 \wedge \frac{k_t(M'_t)}{k_t(M_t)}$$

**end for**
$\phi \leftarrow \phi''$ with probability

$$\begin{aligned} 1 \wedge \quad & \frac{\pi(\phi'')}{\pi(\phi)} \\ \times & \prod_{\{t:\phi_t \neq \phi''_t\}} \frac{f(\phi_t|\phi'_t)}{f(\phi'_t|\phi_t)} \times \frac{1 \wedge \frac{k_t(Q_t)}{k_t(Q'_t)}}{\alpha(\phi_t, \phi'_t)} \\ \times & \prod_{\{t:\phi_t = \phi''_t\}} \frac{1 - 1 \wedge \frac{k_t(Q'_t)}{k_t(Q_t)}}{1 - \alpha(\phi_t, \phi'_t)} \end{aligned}$$

---

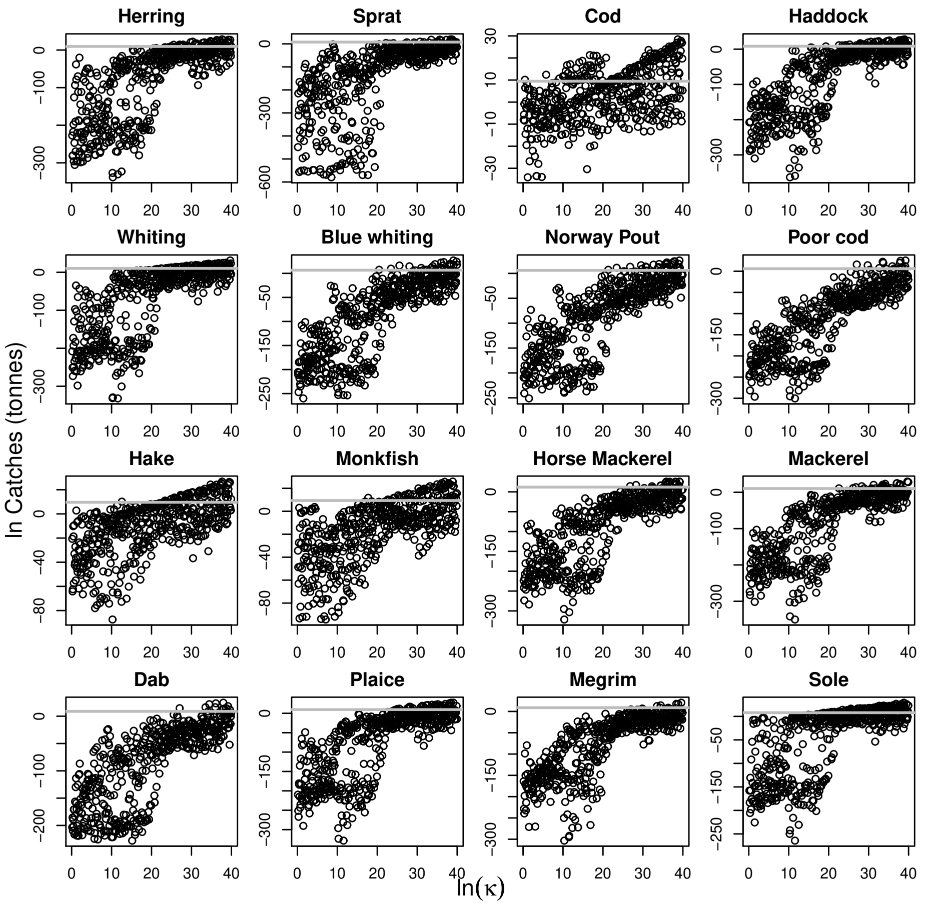


Figure S4: The simulated commercial catches in the first round of history matching against $\ln \kappa$ values. The grey line is the observed catches.

the first year, with the grey line being the observed commercial catches, for different values of $\ln R_{max,1:16}$ and $\phi_{0,1:16}$ when $\ln \kappa > 20$ respectively.

We did another round of history matching, generated using Sobol sequences (Sobol', 1967) with parameter ranges learned from Figures S4, S5 and S6. Figure S7 shows the modelled commercial landing for the first year, with the grey line being the observation, for different values of $\ln \kappa$. From this figure it is clear that $\ln \kappa > 25$. Figures S8 and S9 show the modelled commercial catches for the first year, with the grey line being the observed commercial catches, for different values of $\ln R_{max,1:16}$ and $\phi_{0,1:16}$ when $\ln \kappa > 25$ respectively.

From these plots we decided on the initial parameter values for the MCMC. Table S5 shows the initial values of the MCMC algorithm. $\ln \kappa$ was set to 30 and the boarfish parameters were set to the middle of their

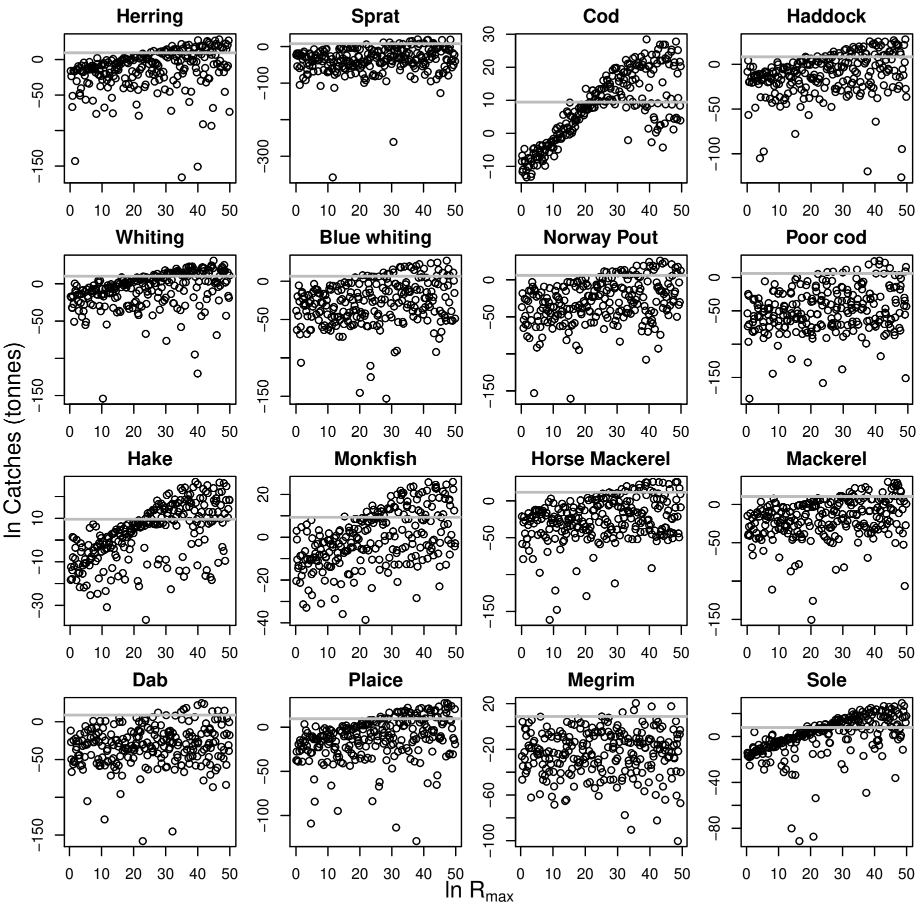


Figure S5: The simulated commercial catches in the first round of history matching with $\ln \kappa > 20$ against $\ln R_{max,i}$ values. The grey line is the observed catches.

prior ranges. To set the initial dynamical parameters we ran Algorithm 2, with the final acceptance probability being

$$1 \wedge \frac{p(\phi''_{1:17,1:24}) l(\boldsymbol{y}|\phi''_{1:17,1:24})}{p(\phi_{1:17,1:24}) l(\boldsymbol{y}|\phi_{1:17,1:24})},$$

1000 times with the initial parameters being $\phi_{1:17,1:24} = 0.75$.

## S4.2 MCMC

We checked the convergence of the MCMC algorithm by visually inspecting the traceplots for all of the parameters. The traceplots for the static parameters $\theta_{1:16}$ and $\theta_{19:34}$ are shown in Figures S10 and S11 respectively.

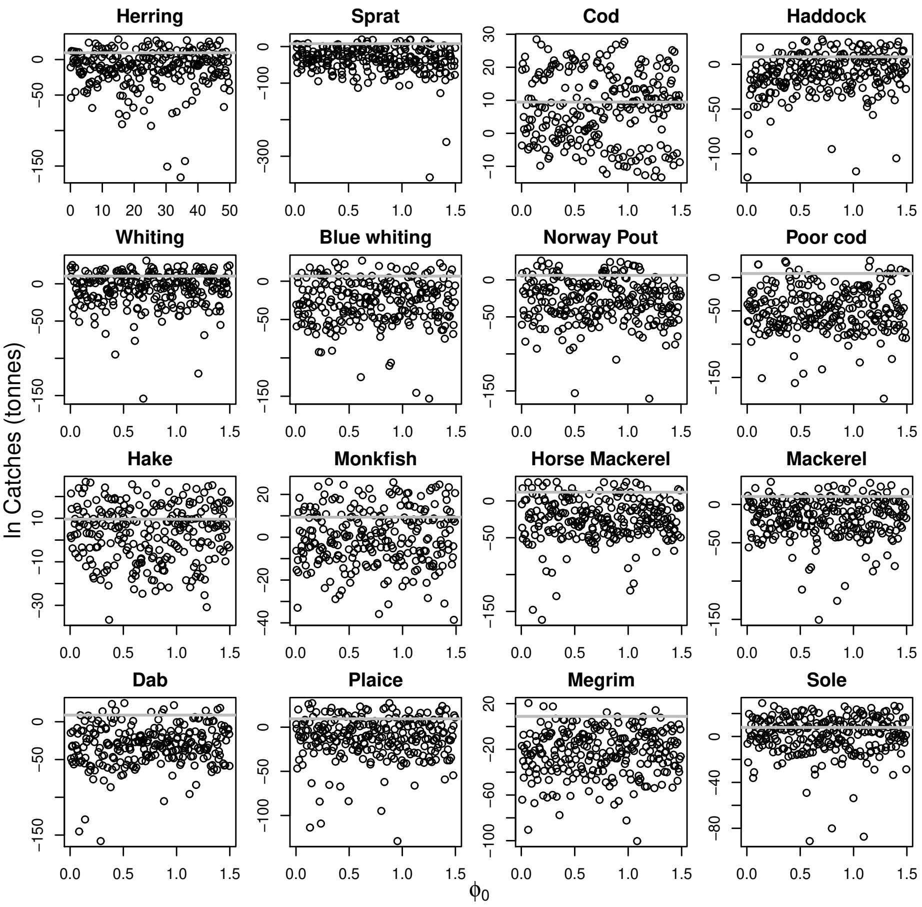


Figure S6: The simulated commercial catches in the first round of history matching with $\ln \kappa > 20$ against $\phi_{0,i}$ values. The grey line is the observed catches.

The dynamical parameters for the first 16 species in the 5th, 10th 15th and 200th year are shown in Figures S12, S13, S14 and S15 respectively.

We ran the beginning of the MCMC algorithm several times and checked visually that the parameters converged in the same location.

## S4.3 Validation

Figure S16 shows the simulated survey catches and the observed survey catches. We investigated the residual patterns from this study. Figures S17 and S18 show the standardised residuals for the commercial catches and the survey catches respectively. Figures S19 and S20 auto correlation function of the commercial catches and the survey catches respectively.

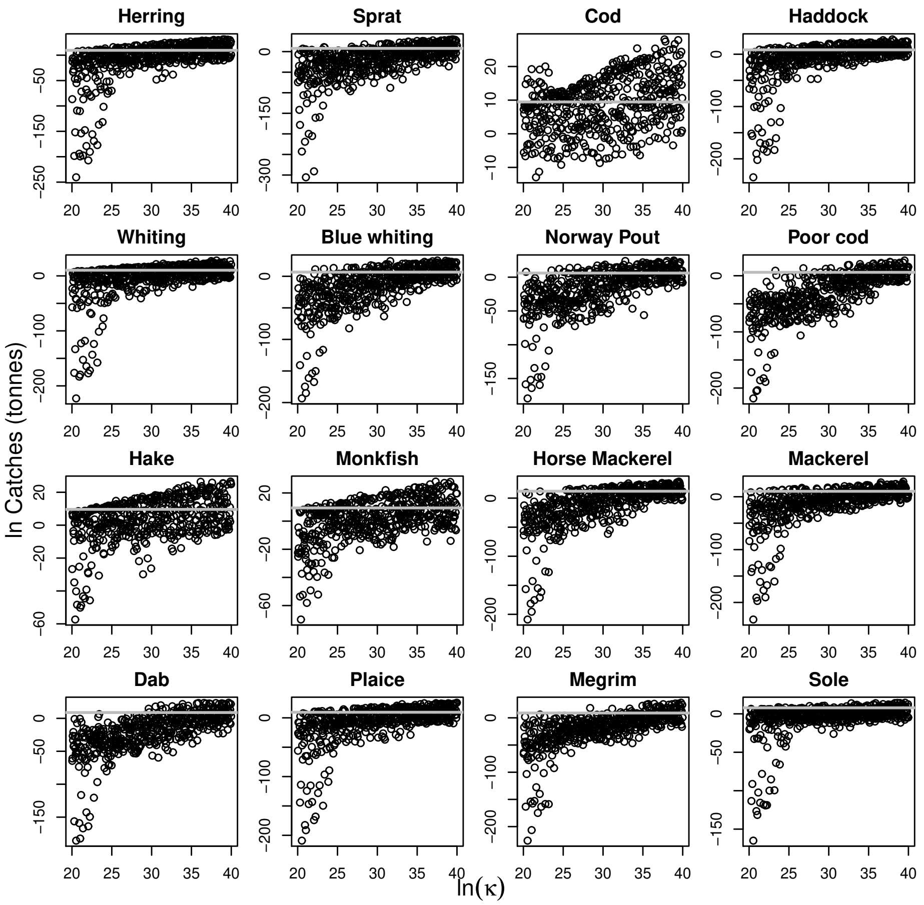


Figure S7: The simulated commercial catches in the second round of history matching against $\ln \kappa$ values. The grey line is the observed catches.

The standardised residuals of the commercial catches are randomly distributed around the Gaussian distribution for most of the species. They appear to be uncorrelated in time, with only really megrim suggesting any auto-correlation in time, suggesting that our assumption of independent errors is not violated. The standardised residuals for the surveys are not always centered on 0. This is often the case in state-space models, because the observations are dependent on one another through the state-space, however we found less correlation between residuals, with the majority of residuals having little auto-correlation suggesting that our assumption of independent errors on the survey data is not violated.

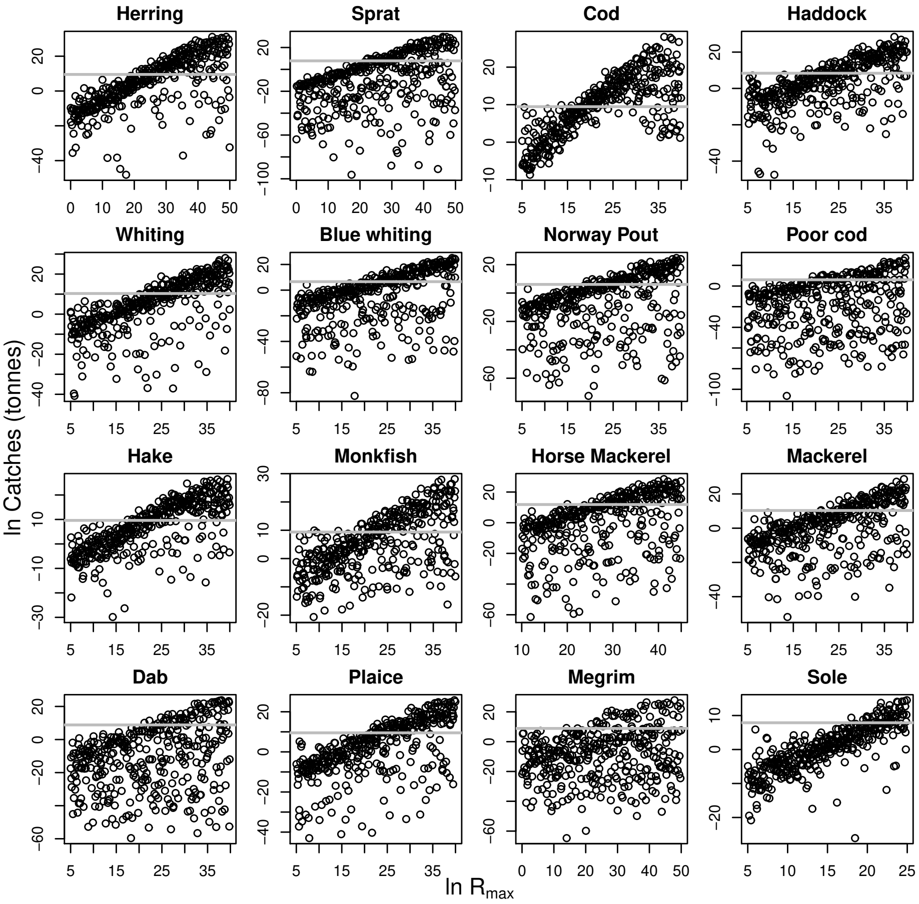


Figure S8: The simulated commercial catches in the second round of history matching with $\ln \kappa > 25$ against $\ln R_{max,i}$ values. The grey line is the observed catches.

# S5 Illustrative example: 'tuning parameters' v 'input variables'

In this example we are going to demonstrate what is meant by 'tuning parameters' and 'input variables' and how they are model specific. We consider an experiment where we drop a tennis ball and observe the time it takes to drop $d$ metres, $t_i$ for $i = 1, \ldots, n$. We assume that we know the error of the stopwatch so that

$$t_i \sim N(t, 0.1^2),$$

where $t$ is the true time, in seconds, it took for the tennis ball to drop.

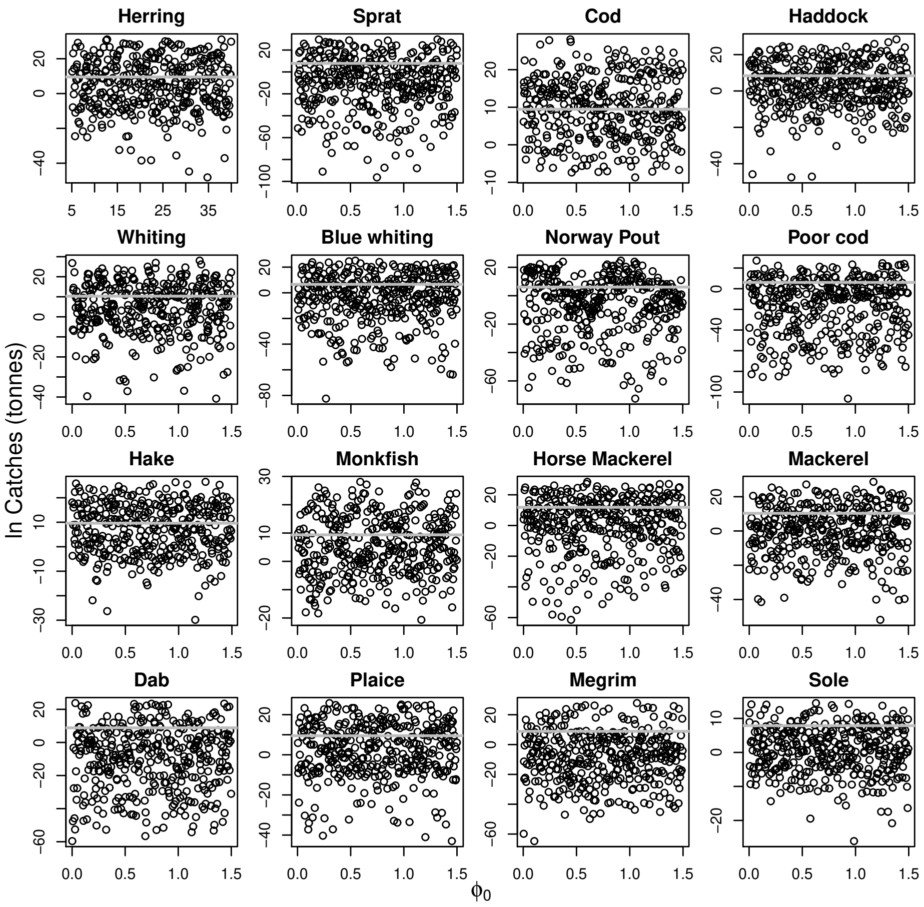


Figure S9: The simulated commercial catches in the second round of history matching with $\ln \kappa > 25$ against $\phi_{0,i}$ values. The grey line is the observed catches.

We have a model for the time taken for an object to fall $d$ meters in a vacuum,

$$t = \sqrt{\frac{2d}{g}}, \tag{S8}$$

where $g$ is the gravitational constant.

Lets first pretend that we do not know $g$. We experimented by dropping a tennis ball from 20 meters and then used the model described in equation S8 to find $g$. Figure S21 shows the posterior density for $n = 5$, 10, 100 and 1000. We get more and more certain about the wrong value of $g$ (the true gravitational constant for Earth is 9.807). This is because we did not drop the tennis ball in a vacuum and therefore the model described by S8

Table S5: The initial static parameters for the MCMC chain. $\ln \kappa$ was set to 30.

| $i$ | Species | $\ln R_{max,i}$ | $\phi_{0,i}$ |
|---|---|---|---|
| 1 | Herring | 21 | 0.75 |
| 2 | Sprat | 20 | 0.75 |
| 3 | Cod | 17 | 0.75 |
| 4 | Haddock | 20 | 0.75 |
| 5 | Whiting | 22 | 0.75 |
| 6 | Blue whiting | 22 | 0.75 |
| 7 | Norway Pout | 22 | 0.75 |
| 8 | Poor cod | 23 | 0.75 |
| 9 | Hake | 21 | 0.75 |
| 10 | Monkfish | 21 | 0.75 |
| 11 | Horse Mackerel | 24 | 0.75 |
| 12 | Mackerel | 22 | 0.75 |
| 13 | Dab | 22 | 0.75 |
| 14 | Plaice | 23 | 0.75 |
| 15 | Megrim | 22 | 0.75 |
| 16 | Sole | 19 | 0.75 |
| 17 | Boarfish | 25 | 0.75 |

is not correct. In this case $g$ is a 'tuning parameter' and it is being used to compensate for both the observation error and the modelling error. It therefore loses all meaning outside of the model. Let us now use the value of $g$ found here as inputs to another model,

$$t = \frac{v_\infty}{g} \text{arcosh}\left(\exp\left(\frac{dg}{v_\infty^2}\right)\right), \tag{S9}$$

where $v_\infty$ is the terminal velocity of the tennis ball (which is about 30m/s). We now use the posterior mean for $g$ (9.087) as an 'input variable' and calculate how long it would take for a tennis ball to drop 30 meters. We calculate it to be 2.701 seconds when in fact it would take 2.610 if we were to use the correct value of $g$. This is an example of the model error in equation S8 causing an error in the model described by equation S9 caused by attaching a meaning to a 'tuning parameter' and using it as an 'input variable' to another model.

# References

Julia L. Blanchard, Ken H. Andersen, Finlay Scott, Niels T. Hintzen, Gerjan Piet, and Simon Jennings. Evaluating targets

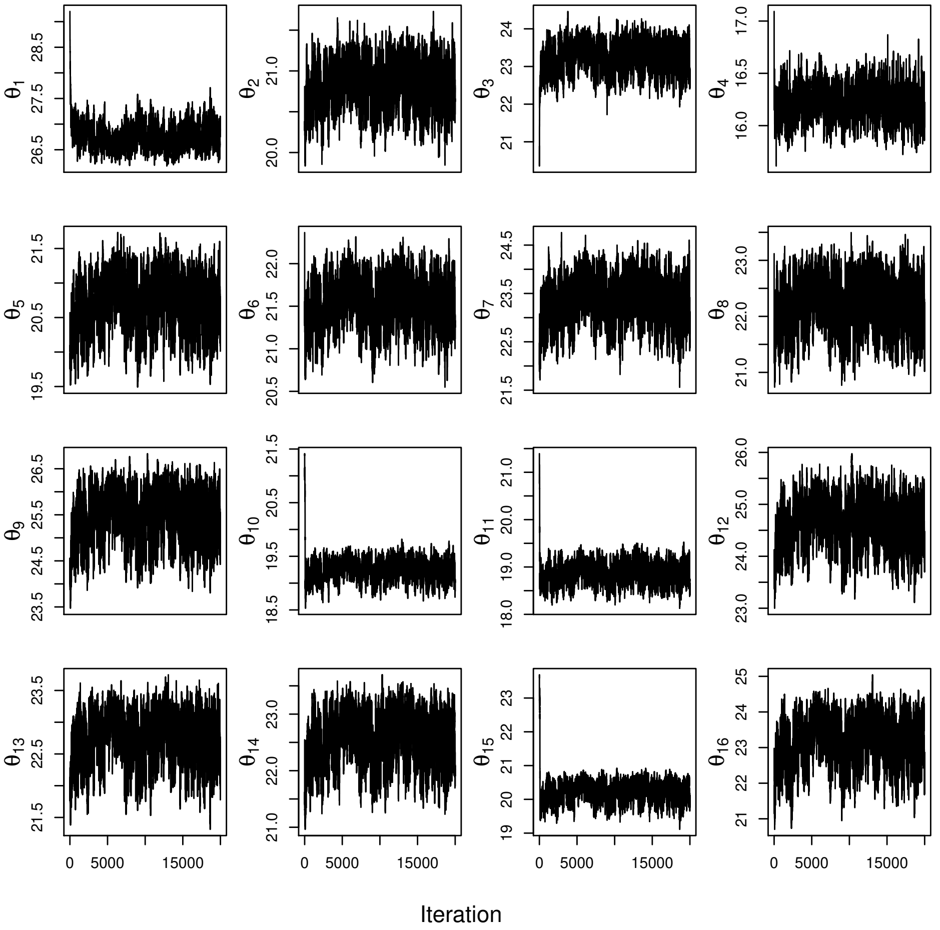


Figure S10: The traceplots of the MCMC for the static parameters $\theta_{1:16}$, which includes $\ln \kappa$ and $\ln R_{max,1:15}$.

and trade-offs among fisheries and conservation objectives using a multispecies size spectrum model. *Journal of Applied Ecology*, 51(3):612–622, 2014. doi: 10.1111/1365-2664.12238. URL `https://besjournals.onlinelibrary.wiley.com/doi/abs/10.1111/1365-2664.12238`.

Ben Calderhead. A general construction for parallelizing Metropolis-Hastings algorithms. *Proceedings of the National Academy of Sciences*, 111 (49):17408–17413, 2014. ISSN 0027-8424. doi: 10.1073/pnas.1408184111. URL `http://www.pnas.org/content/111/49/17408`.

Tiangang Cui, Colin Fox, Geoff Nicholls, and Michael O'Sullivan. Using Parallel MCMC Sampling to Calibrate a Computer Model of a Geothermal reservoir. Technical report, Report University of Auckland Faculty of Engineering 686, 01 2011.

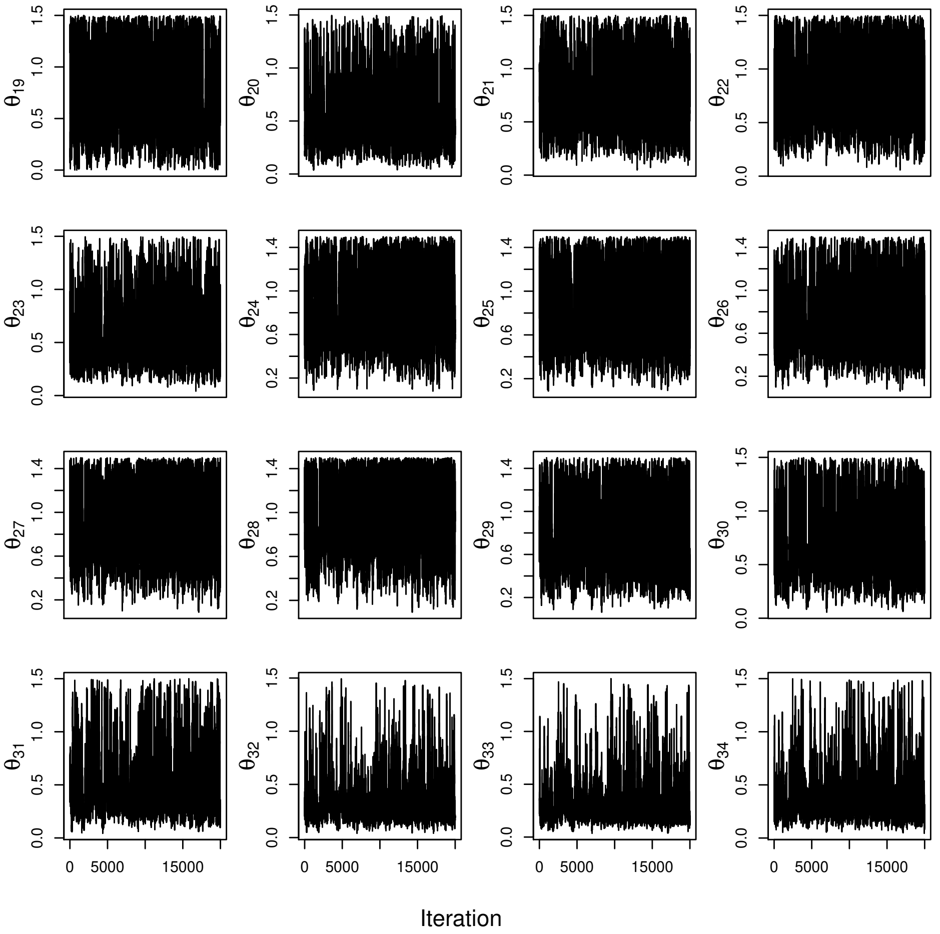


Figure S11: The traceplots of the MCMC for the static parameters $\theta_{19:34}$, which is $\phi_{0,1:16}$

Martin Hartvig, Ken H. Andersen, and Jan E. Beyer. Food web framework for size-structured populations. *Journal of Theoretical Biology*, 272(1):113 – 122, 2011. ISSN 0022-5193. doi: https://doi.org/10.1016/j.jtbi.2010.12.006. URL `http://www.sciencedirect.com/science/article/pii/S0022519310006612`.

ICES. Database of Trawl Surveys (DATRAS), 2017. http://datras.ices.dk.

Finlay Scott, Julia L. Blanchard, and Ken H. Andersen. mizer: an R package for multispecies, trait-based and community size spectrum ecological modelling. *Methods in Ecology and Evolution*, 5(10):1121–1125, 2014. doi: 10.1111/2041-210X.12256. URL `https://besjournals.onlinelibrary.wiley.com/doi/abs/10.1111/2041-210X.12256`.

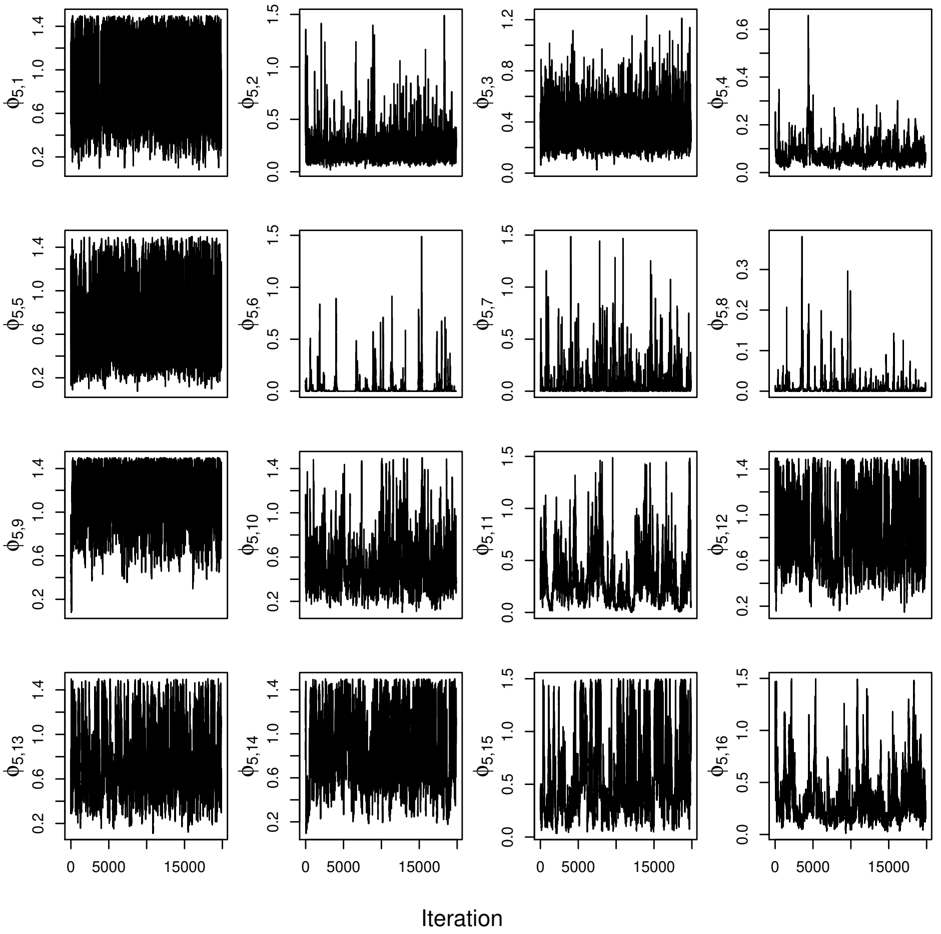

Figure S12: The traceplot of the MCMC for the dynamic parameters, $\phi_{5,1:16}$.


I.M Sobol'. On the distribution of points in a cube and the approximate evaluation of integrals. *USSR Computational Mathematics and Mathematical Physics*, 7(4):86 – 112, 1967. ISSN 0041-5553. doi: https://doi.org/10.1016/0041-5553(67)90144-9. URL `http://www.sciencedirect.com/science/article/pii/0041555367901449`.

Michael A. Spence, Paul G. Blackwell, and Julia L. Blanchard. Parameter uncertainty of a dynamic multispecies size spectrum model. *Canadian Journal of Fisheries and Aquatic Sciences*, 73(4):589–597, 2016. doi: 10.1139/cjfas-2015-0022.

Nicola D. Walker, David L. Maxwell, Will J. F. Le Quesne, and Simon Jennings. Estimating efficiency of survey and commercial trawl gears from comparisons of catch-ratios. *ICES Journal of Marine Sci-*

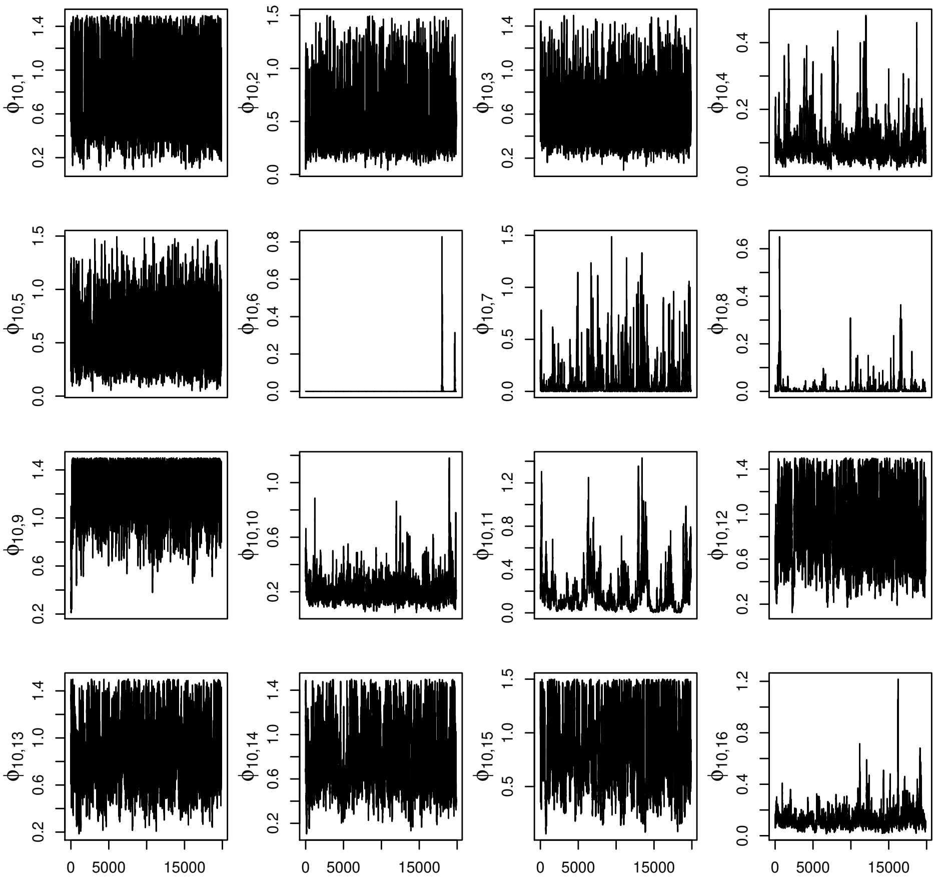

Figure S13: The traceplot of the MCMC for the dynamic parameters, $\phi_{10,1:16}$.

*ence*, 74(5):1448–1457, 2017. doi: 10.1093/icesjms/fsw250. URL `http://dx.doi.org/10.1093/icesjms/fsw250`.

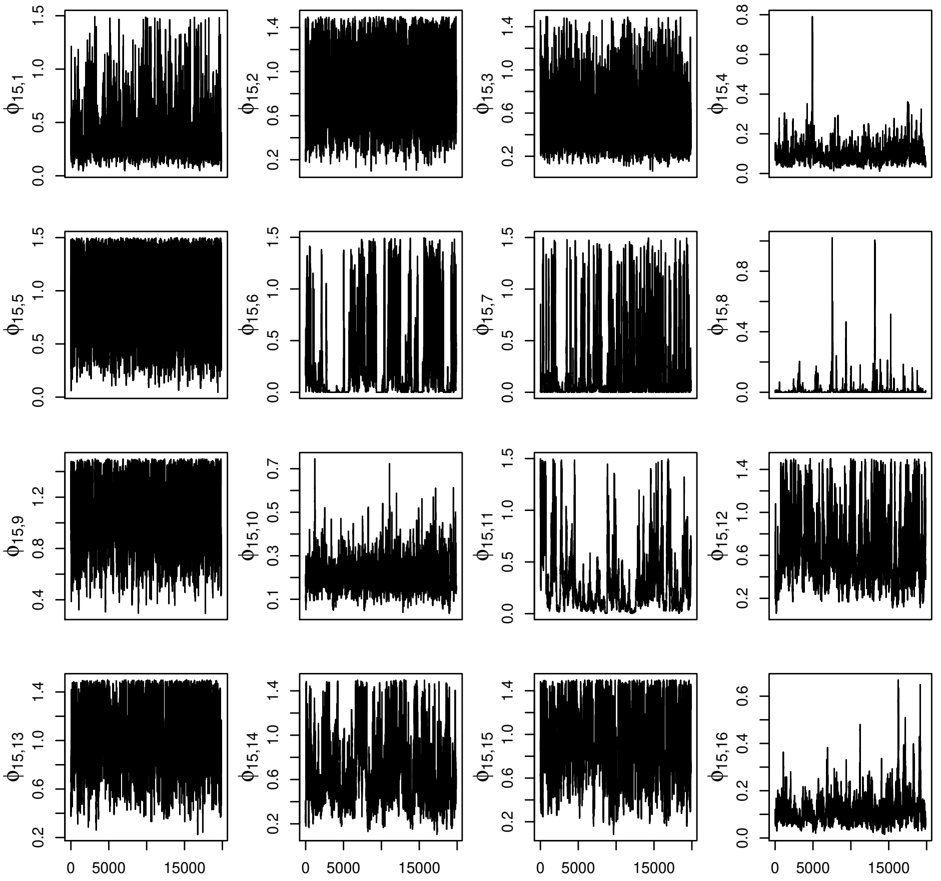


Figure S14: The traceplot of the MCMC for the dynamic parameters, $\phi_{15,1:16}$.

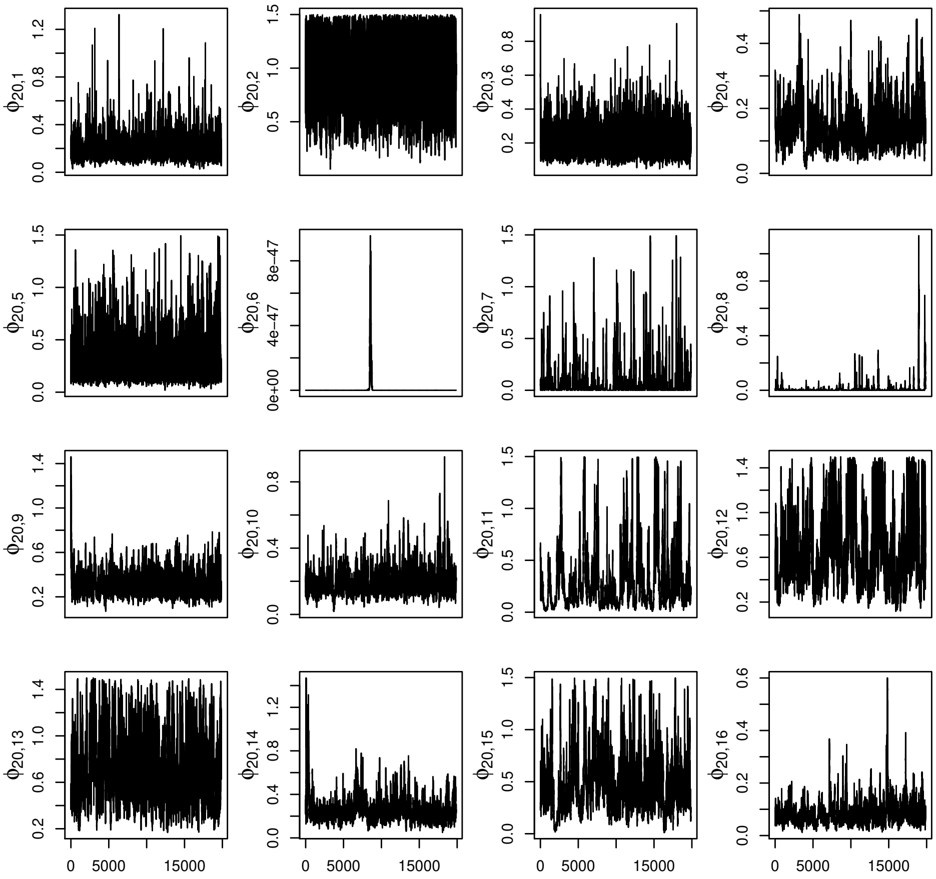


Figure S15: The traceplot of the MCMC for the dynamic parameters, $\phi_{20,1:16}$.

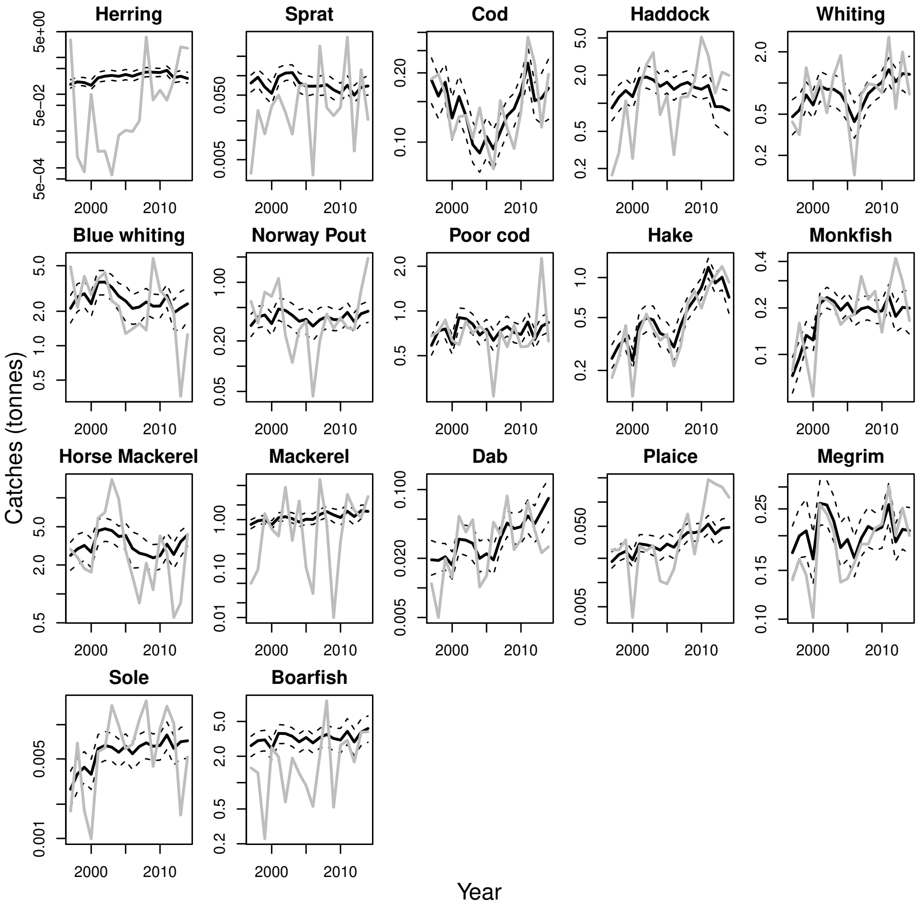


Figure S16: The median modelled survey catches (solid black line), the 10th and 90th percentiles (dotted black lines) and the observed catches (grey line).

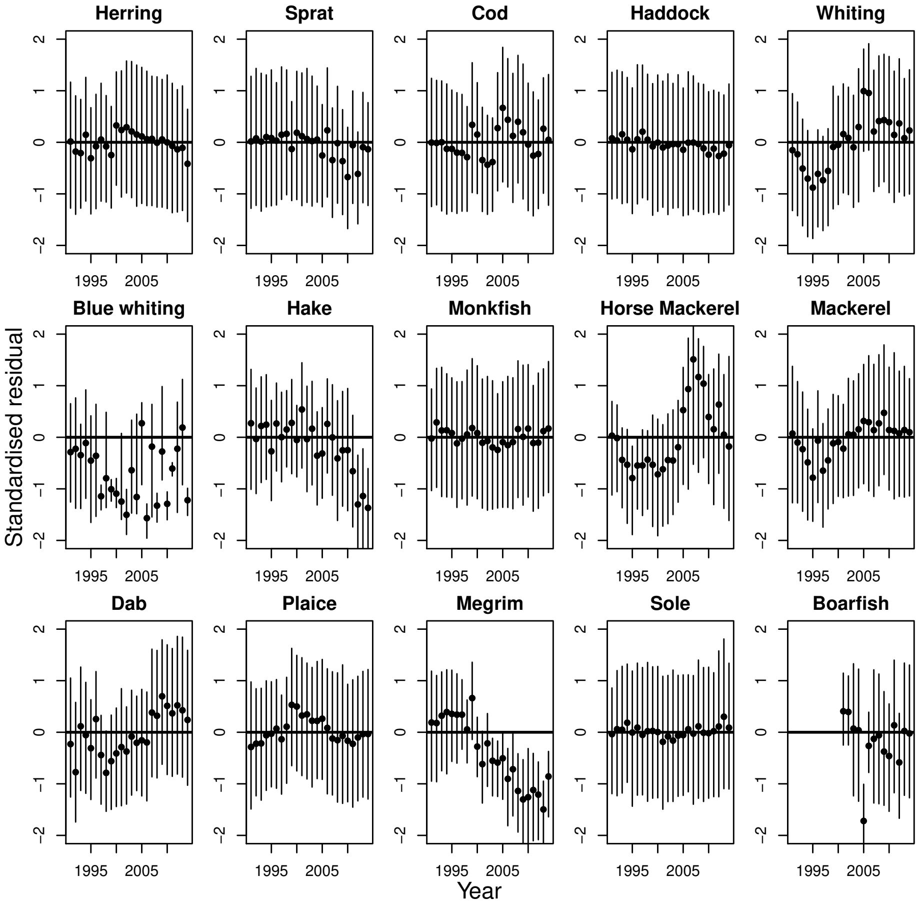


Figure S17: The standardised residuals of the commercial catches. The point is the median and the line is from the 10th and 90th percentiles.

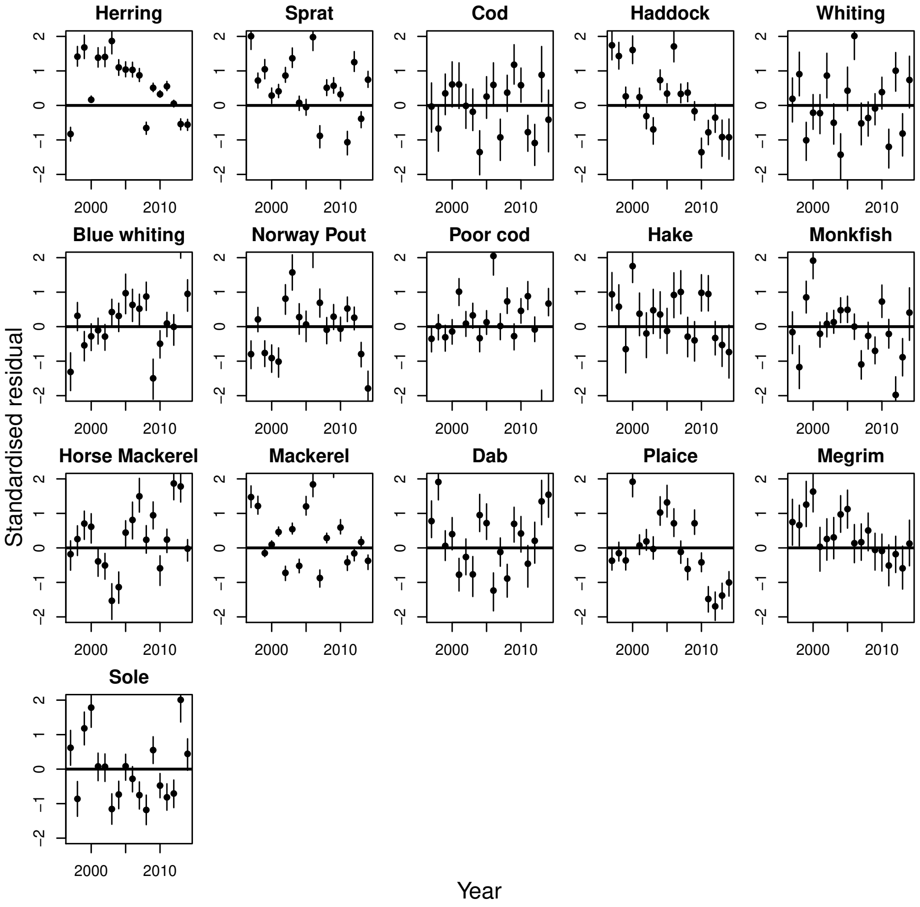


Figure S18: The standardised residuals of the survey catches. The point is the median and the line is from the 10th and 90th percentiles.

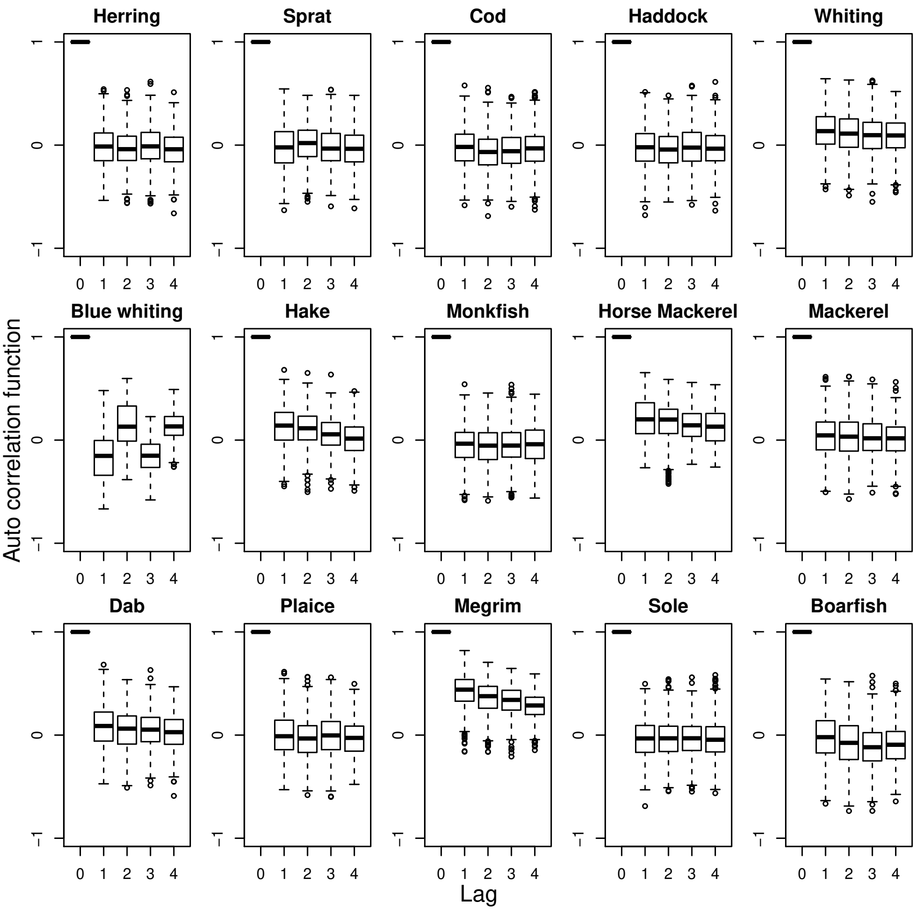


Figure S19: The auto correlation function of the standardised residuals of the commercial catches.

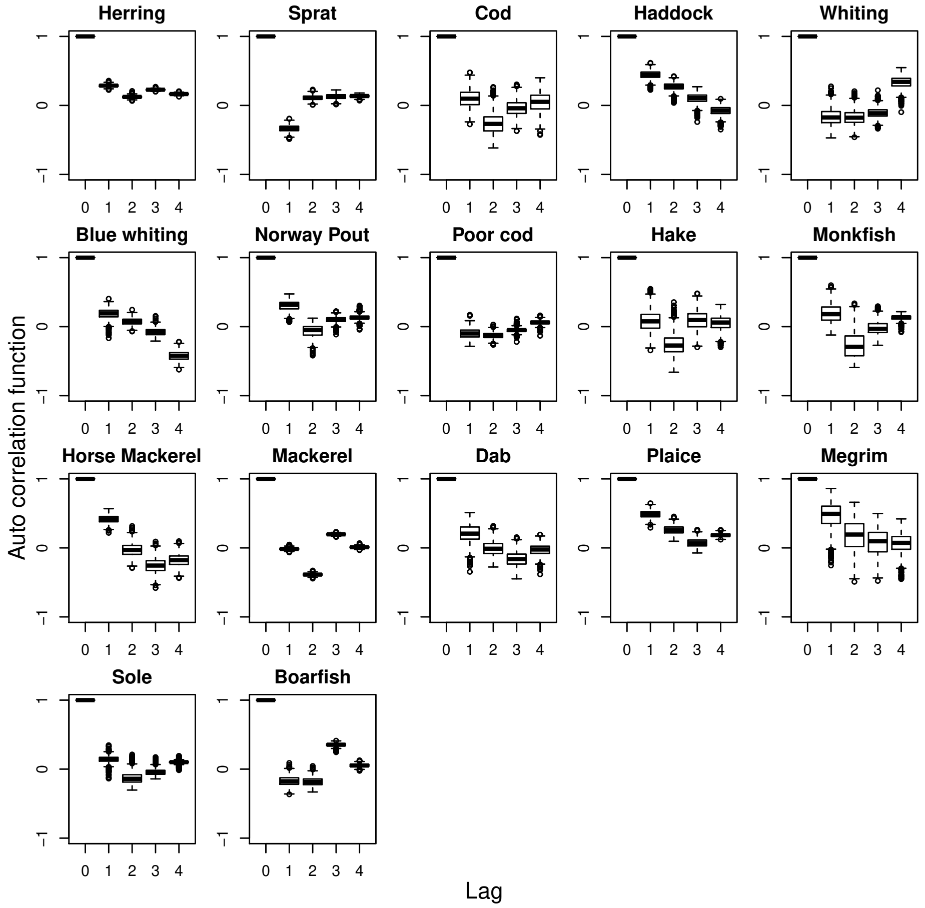


Figure S20: The auto correlation function of the standardised residuals of the survey catches.

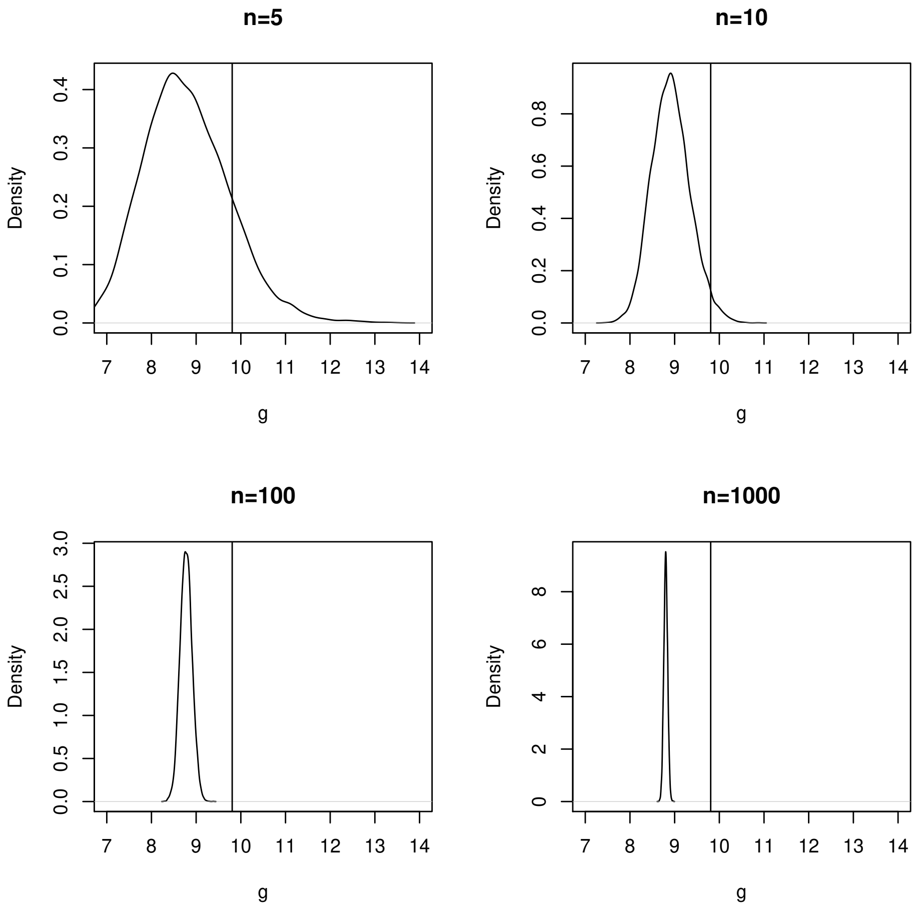


Figure S21: The posterior distribution of $g$ from the model described in equation S8 for $n$ observations. The solid line is the true value of the gravitational constant for Earth, 9.807.
