# Supplementary material for: Quantifying uncertainty and dynamical changes in multi-species fishing mortality rates, catches and biomass by combining state-space and mechanistic multi-species models
Source: arXiv:2008.02765 ancillary file (2020-08-06)
Supplement: Supplementary file 2 [file Simulation_study.pdf]

# Simulation study

Michael A. Spence

30/07/2020

## Introduction

In this document I demonstrate a simulation study that uses the methods described in the manuscript to fit a simulated example using the LeMans model (Thorpe et al. 2015) with 3 species. For a complete description of the model see Spence (2020). I ran the model for 20 years and observed the commercial catches,  $w_{i,t}$ , and survey catches,  $z_{i,t}$ , for each species  $i = 1, 2, 3$  and year  $t = 1, \dots, 20$ . The uncertain static parameters are  $b_i$  (or **b**) from the **hockey stick** recruitment curve;  $\phi_{0,i}$  (or **spinupF**), the fishing mortality during the spin up period and  $\kappa$  (or **other**), the other food available in the system. In addition I am interested in the dynamical parameters, the fishing rates for the 20 species each year,  $\phi_{t,i}$ , for  $t = 1 \dots 20$  and  $i = 1, 2, 3$ .

The likelihood of the model is

$$\prod_{t=1}^{20} \prod_{i=1}^3 N(\ln(w_{i,t}) | \ln(c(M_{i,t}(\theta, \phi_{1:20,1:3}))), \sigma_{c,i}^2) N(\ln(z_{i,t}) | \ln(b(M_{i,t}(\theta, \phi_{1:20,1:3}))), \sigma_{s,i}^2),$$

where  $c(M_{i,t}(\theta, \phi_{1:20,1:3}))$  is the commercial catch of the  $i$ -th species in the  $t$ -th year,  $b(M_{i,t}(\theta, \phi_{1:20,1:3}))$  is the survey catch of the  $i$ -th species in the  $t$ -th year,  $\theta = (\ln(\kappa), \ln(b_1), \ln(b_2), \ln(b_3), \phi_{0,1}, \phi_{0,2}, \phi_{0,3})$  and  $N(a|d, e)$  is a normal density with expectation  $d$  and variance  $e$  evaluated at  $a$ .  $\sigma_{c,i}^2$  and  $\sigma_{s,i}^2$  will be estimated.

I believed that  $\ln(\kappa) \in (0, 30)$ ,  $\ln(b_i) \in (0, \infty)$  and  $\phi_{t,i}$  for  $i = 1, 2, 3$  and  $t = 0, 1, \dots, 20$ . I also believed

$$\sigma_{c,i}^2 \sim \text{Inv-Gamma}(0.1, 0.1)$$

and

$$\sigma_{s,i}^2 \sim \text{Inv-Gamma}(0.1, 0.1)$$

for  $i = 1, 2, 3$ .

## Simulating the data

First I load the package and setup a model with only three species in it, sprat, mackerel and cod:

```
library(LeMaRns)
set.seed(14)
spec_par <- NS_par[c(1,11,20),]
tau <- NS_tau[c(1,11,20),c(1,11,20)]
spec_par$a <- exp(17.429 - 3.792 * log(spec_par$Linf))
```

The set of the parameters that I am going to try and fit.

```
spec_par$b <- exp(c(11,7.5,1))
```

therefore the true value of  $\theta_{2:4}$  will be  $c(11,7.5,1)$ . I then setup the model with  $\theta_1$  equal to 27:

```
params <- LeMansParam(spec_par, tau=tau, eta=rep(0.25, 3), L50=spec_par$Lmat, other=exp(27))
```

and the effort matrix for the spin-up period, which in this case is 100 years:

```
effort <- matrix(c(0.1,0.3,0.6), 100, dim(params@Qs)[3], byrow = T)
```

The fishing effort during the spin up period,  $\theta_{5:7}$  is  $c(0.1,0.3,0.6)$  for each of the three species, a parameter I am interested in fitting. I simulate the spin up period:

```
model_run <- run_LeMans(params, years=100, effort=effort)
```

For the fishing period I need to add the survey vessel. I use data from Walker et al. (2017) and setup the gear selection:

```
custom_q <- matrix(0,32,3)
custom_q[,1] <- c(0.017254858,0.043039643,0.284392929,rep(0.430695848,29))
custom_q[,2] <- c(0.096113412,rep(0.24028353,31))
custom_q[,3] <- c(0.001761793,0.006166274,0.039181631,0.092776614,0.145237111,0.193340804,
0.232928633,0.2564465,0.27551981,0.28422822,0.290723986,0.296690919,
0.305572708,0.316083176,0.334233041,0.358307207,0.388331838,0.416365328,
0.455782759,0.499352575,0.536897304,0.587032109,0.640318341,0.695650091,
0.740381939,0.740381939,0.740381939,0.740381939,0.740381939,0.740381939,
0.740381939,0.740381939)
)
params@Qs <- abind::abind(params@Qs,custom_q)
dimnames(params@Qs)[[3]][4] <- "survey"
```

I am going to run a 20 year time series with fishing effort and survey effort:

```
Fs <- abs(cbind(abs(cumsum(rnorm(20,0,0.075)) + 0.1),cumsum(rnorm(20,0,0.075))
+ 0.6,cumsum(rnorm(20,0,0.075)) + 0.25))
sur_ef <- abs(rnorm(20,0.0001,0.0001))
fish_rate <- as.matrix(cbind(Fs,sur_ef));colnames(fish_rate) <- NULL
```

The fishing effort is

```
Fs
```

```
##           [,1]      [,2]      [,3]
## [1,] 0.05036126 0.5049889 0.217661922
## [2,] 0.17928282 0.4900951 0.246345413
## [3,] 0.33840785 0.5005101 0.249429795
## [4,] 0.45069438 0.4795599 0.244987995
## [5,] 0.44798383 0.5327288 0.147756196
## [6,] 0.54037972 0.4752331 0.012517032
## [7,] 0.53551366 0.5834853 0.079538134
## [8,] 0.61568819 0.6468512 0.033583168
## [9,] 0.58741579 0.6168984 0.010139674
## [10,] 0.66565453 0.5098159 0.009698523
## [11,] 0.63694289 0.4031664 0.130210131
## [12,] 0.65939950 0.3785493 0.007038693
## [13,] 0.70996749 0.3998921 0.067294999
## [14,] 0.68800626 0.4538423 0.176077596
## [15,] 0.72461026 0.4862735 0.177189453
## [16,] 0.79082040 0.4598791 0.136941524
## [17,] 0.93052657 0.4822082 0.197774306
## [18,] 1.05140597 0.4626008 0.221648666
## [19,] 1.06156694 0.5607525 0.138287966
## [20,] 1.14317339 0.5619428 0.148918819
```

I then simulate the catch data:

```
model_run_act <- run_LeMans(params, years=20, effort=fish_rate,NO=model_run@N[,1001])
plot_biomass(params,model_run_act)
```

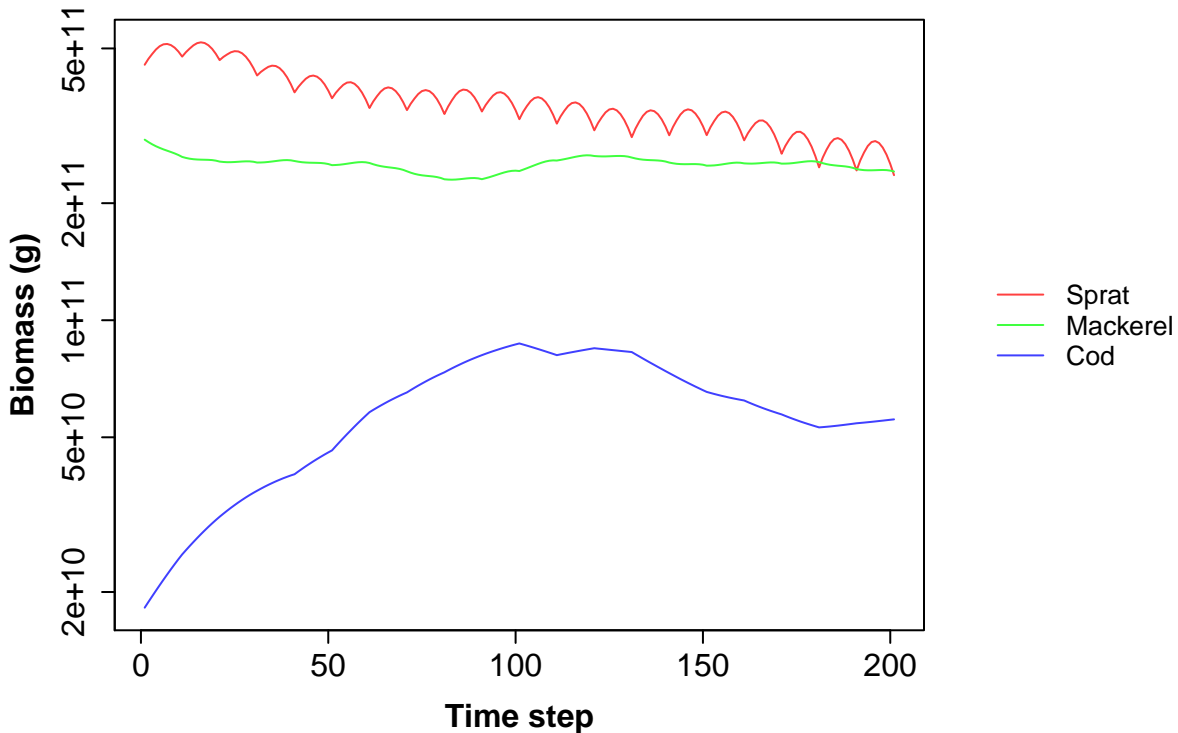

```
catches <- get_CPG(params,model_run_act,effort=fish_rate)
com_catches_t <- apply(catches[,1:3,],c(2,3),sum)
sur_catch <- com_catches <- matrix(0,20,3)
for (i in 1:20){
  com_catches[i,] <- log(rowSums(com_catches_t[,10 * (i-1) + (1:10)])) - log(1e6)
  sur_catch[i,] <- log(rowSums(catches[,4,10 * (i-1) + (1:10)])) - log(1e6)
}
```

and add some stochasticity to the catches

```
sigma_c <- c(0.38,0.44,0.5); sigma_s <- c(0.6,0.7,0.6)
obs_c <- com_catches + matrix(rnorm(60,0,sigma_c),20,3,byrow=T)
obs_s <- sur_catch + matrix(rnorm(60,0,sigma_s),20,3,byrow=T)
```

The observations are:

```
par(mfrow=c(3,2))
plot(1:20,obs_c[,1],main="Sprat",ylab="log commercial catches",type="l")
plot(1:20,obs_s[,1],main="Sprat",ylab="log survey catches",type="l")
plot(1:20,obs_c[,2],main="Mackerel",ylab="log commercial catches",type="l")
plot(1:20,obs_s[,2],main="Mackerel",ylab="log survey catches",type="l")
plot(1:20,obs_c[,3],main="Cod",ylab="log commercial catches",type="l")
plot(1:20,obs_s[,3],main="Cod",ylab="log survey catches",type="l")
```

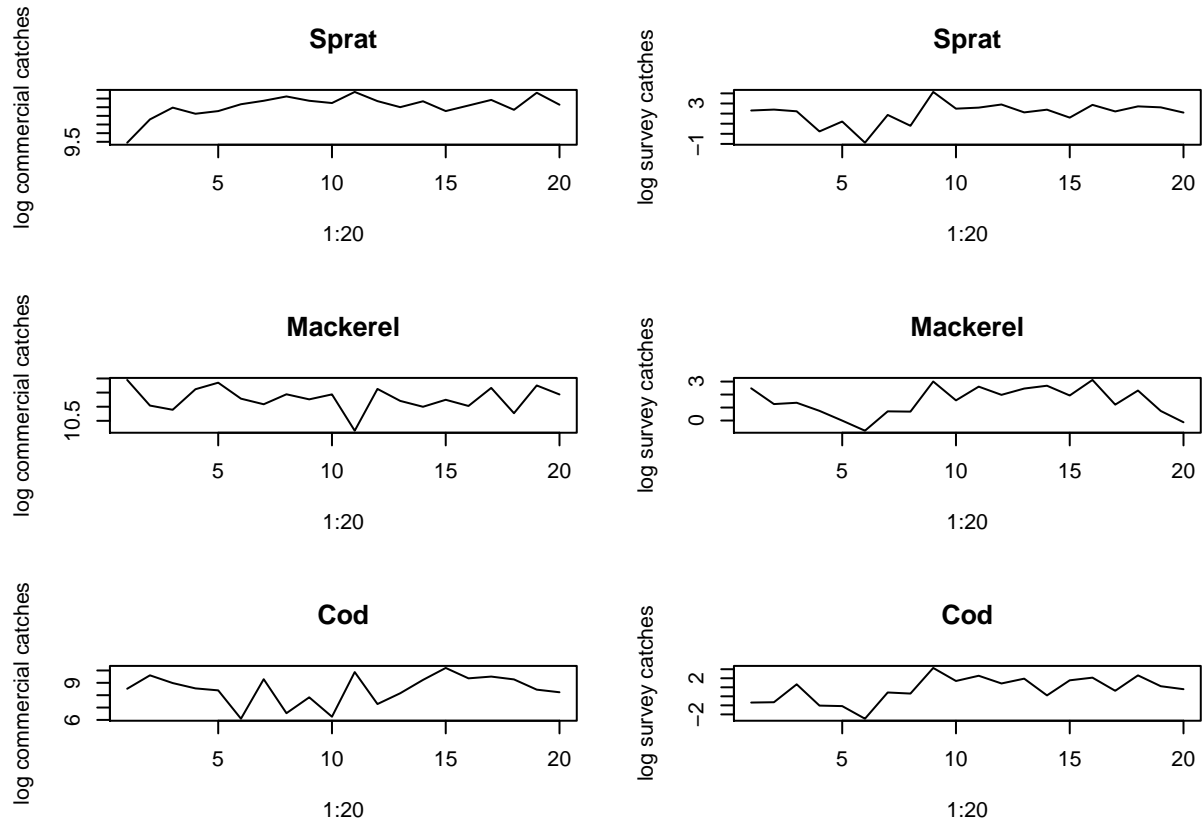

## History matching

To do the history matching to find initial values for the MCMC algorithm I first need to setup two functions. The first takes a model output and calculates the catches:

```
calc_catch <- function(params,model_run,effort){
  catches <- get_CPG(params,model_run,effort=effort)
  com_catches_t <- apply(catches[,1:3,],c(2,3),sum)
  times <- (dim(model_run@N)[3] - 1)*params@phi_min
  sur_catch <- com_catches <- matrix(0,times,3)
  for (i in 1:times){
    com_catches[i,] <- log(rowSums(com_catches_t[,10 * (i-1) + (1:10)])) - log(1e6)
    sur_catch[i,] <- log(rowSums(catches[,4,10 * (i-1) + (1:10)])) - log(1e6)
  }
  return(list(com=com_catches,sur=sur_catch))
}
```

and the second takes in the uncertain static parameters,  $\theta$  and the fishing rates of the first year and outputs the simulated catches from the first year,  $F_{1,i}$ :

```
hist_mat <- function(input,params){
  params@other <- exp(input[1])
  params@recruit_params[[1]][2] <- exp(input[2])
  params@recruit_params[[2]][2] <- exp(input[3])
  params@recruit_params[[3]][2] <- exp(input[4])
  model_run <- run_LeMans(params, years=100, effort=t(matrix(c(input[5:7],0),4,100)))
}
```

```

model_run1 <- run_LeMans(params,years=1,effort=t(matrix(c(input[8:10],sur_ef[1]),4,1)),
                      NO=model_run@N[,dim(model_run@N)[3]])
effort <- t(matrix(c(input[8:10],sur_ef[1]),4,1))
return(unlist(calc_catch(params,model_run1,effort)))
}

```

I now need to generate parameter values for the first round of the history matching using Sobol' indices Sobol' (1967) and run them:

```

library(randtoolbox) ## for sobol indicies
sam1 <- sobol(5000,3*3 + 1)
## other - between 20 and 30
sam1[,1] <- sam1[,1] *20 +10
## b between 0 and 20
sam1[,2:4] <- sam1[,2:4] * 20
## spin-up F and first year fishing mortality between 0 and 1.5
sam1[,5:10] <- sam1[,5:10] * 1.5
library(pbapply) ## do in parallel
round1 <- pbapply(sam1,1,hist_mat,params=params)

```

I then compare the difference between the observed values and the simulated values

```

c_r1 <- round1 - c(obs_c[1,],obs_s[1,])

```

I evaluate the results

```

par(mfrow=c(2,3))
plot(sam1[,1],c_r1[1,],ylim=c(-10,10),xlab="other",ylab="sprat difference",
     main="Commercial catches")
abline(h=0,col="red")
plot(sam1[,1],c_r1[2,],ylim=c(-10,10),xlab="other",ylab="mackerel difference",
     ,main="Commercial catches")
abline(h=0,col="red")
plot(sam1[,1],c_r1[3,],ylim=c(-10,10),xlab="other",ylab="cod difference",
     main="Commercial catches")
abline(h=0,col="red")
plot(sam1[,1],c_r1[4,],ylim=c(-10,10),xlab="other",ylab="sprat difference",
     main="Survey catches")
abline(h=0,col="red")
plot(sam1[,1],c_r1[5,],ylim=c(-10,10),xlab="other",ylab="mackerel difference",
     main="Survey catches")
abline(h=0,col="red")
plot(sam1[,1],c_r1[6,],ylim=c(-10,10),xlab="other",ylab="cod difference",
     main="Survey catches")
abline(h=0,col="red")

```

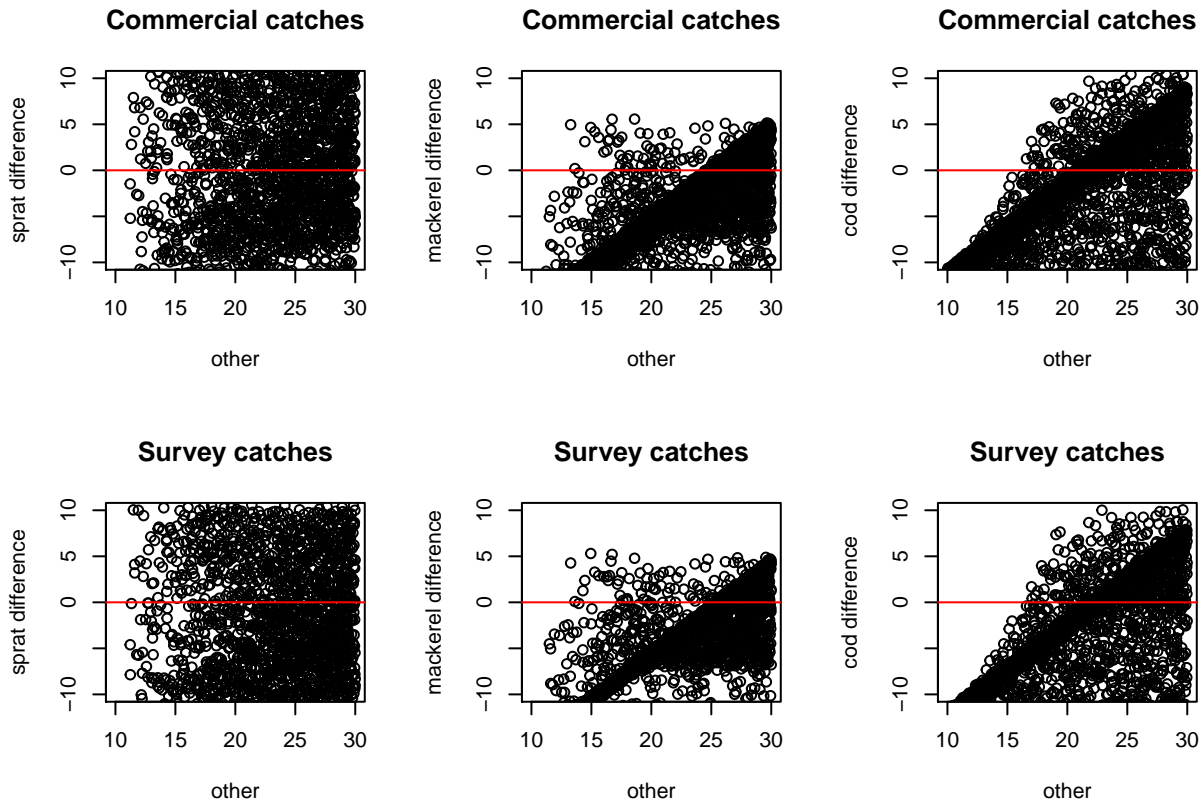

This implies that  $\theta_1$  has to be larger than 24. For  $\theta_{2:4}$ :

```
par(mfrow=c(2,3))
plot(sam1[,2],c_r1[1,],ylim=c(-10,10),xlab="sprat b",ylab="sprat difference",
     main="Commercial catches")
abline(h=0,col="red")
plot(sam1[,3],c_r1[2,],ylim=c(-10,10),xlab="mackerel b",ylab="mackerel difference",
     main="Commercial catches")
abline(h=0,col="red")
plot(sam1[,4],c_r1[3,],ylim=c(-10,10),xlab="cod b",ylab="cod difference",
     main="Commercial catches")
abline(h=0,col="red")
plot(sam1[,2],c_r1[4,],ylim=c(-10,10),xlab="sprat b",ylab="sprat difference",
     main="Survey catches")
abline(h=0,col="red")
plot(sam1[,3],c_r1[5,],ylim=c(-10,10),xlab="mackerel b",ylab="mackerel difference",
     main="Survey catches")
abline(h=0,col="red")
plot(sam1[,4],c_r1[6,],ylim=c(-10,10),xlab="cod b",ylab="cod difference",
     main="Survey catches")
abline(h=0,col="red")
```

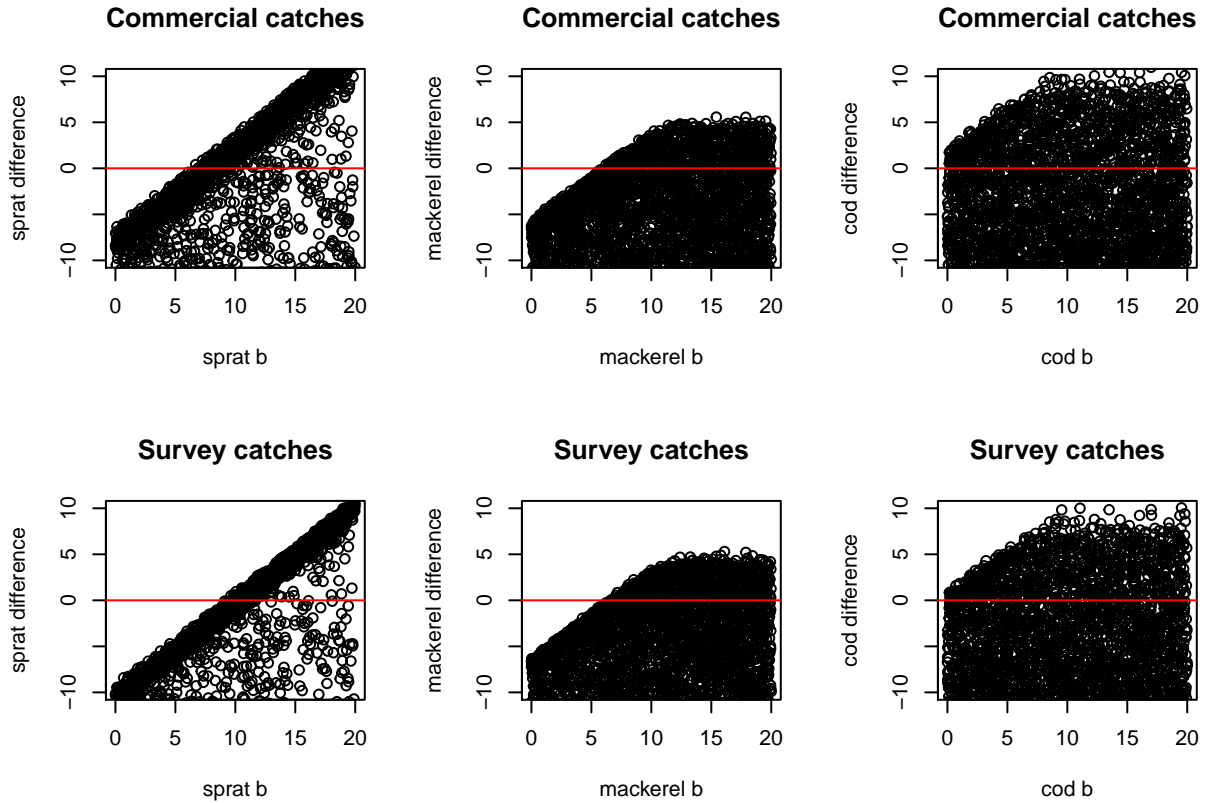

which implies that  $\theta_{2:4}$  needs to be larger than 7, 6 and 0 for sprat, mackerel and cod respectively. For  $\theta_{5:7}$ :

```
par(mfrow=c(2,3))
plot(sam1[,5],c_r1[1,],ylim=c(-10,10),xlab="Spin up F sprat",ylab="sprat difference",
     main="Commercial catches")
abline(h=0,col="red")
plot(sam1[,6],c_r1[2,],ylim=c(-10,10),xlab="Spin up F mackerel",ylab="mackerel difference",
     main="Commercial catches")
abline(h=0,col="red")
plot(sam1[,7],c_r1[3,],ylim=c(-10,10),xlab="Spin up F cod",ylab="cod difference",
     main="Commercial catches")
abline(h=0,col="red")
plot(sam1[,5],c_r1[4,],ylim=c(-10,10),xlab="Spin up F sprat",ylab="sprat difference",
     main="Survey catches")
abline(h=0,col="red")
plot(sam1[,6],c_r1[5,],ylim=c(-10,10),xlab="Spin up F mackerel",ylab="mackerel difference",
     main="Survey catches")
abline(h=0,col="red")
plot(sam1[,7],c_r1[6,],ylim=c(-10,10),xlab="Spin up F cod",ylab="cod difference",
     main="Survey catches")
abline(h=0,col="red")
```

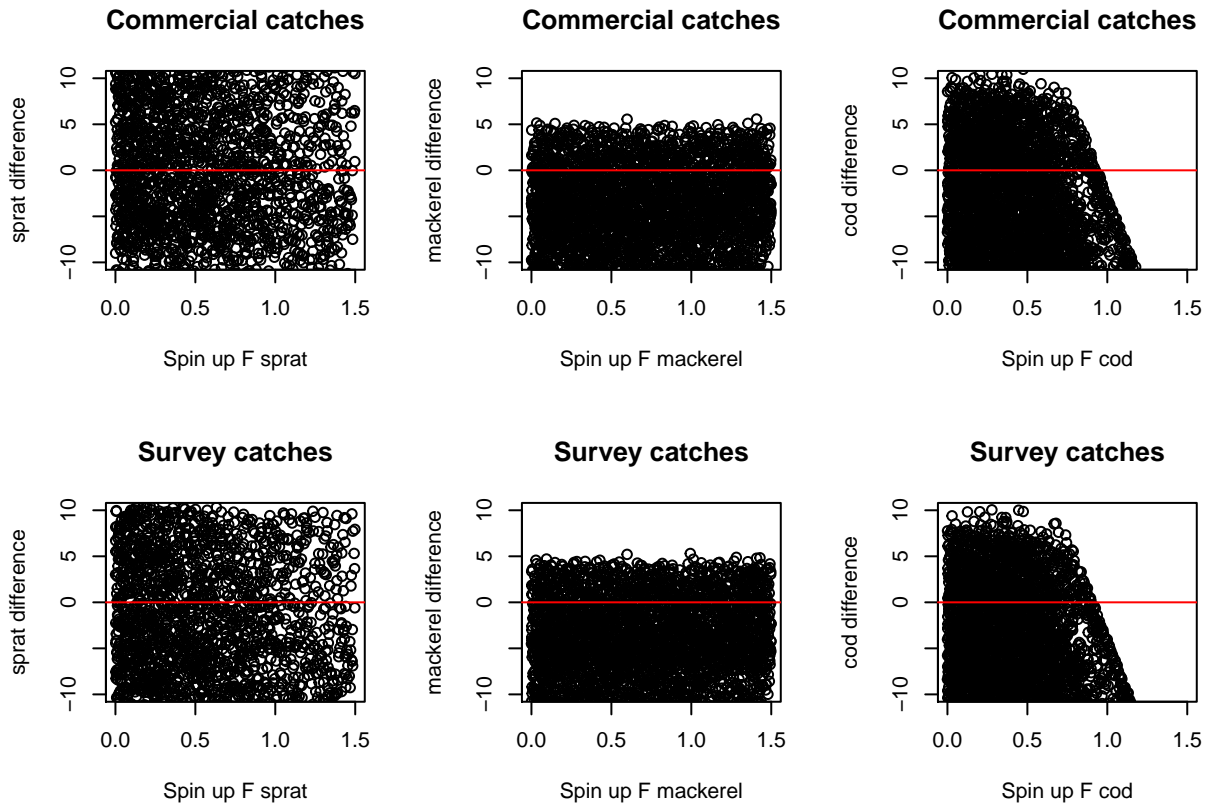

This shows that  $\theta_7$ , the value for cod, must be less than one. To confirm this I will run a second round.

```
sam2 <- sobol(5000,3*3 + 1,init = F)
sam2[,1] <- sam2[,1] * 6 + 24
sam2[,2:4] <- t(t(sam2[,2:4]) * c(13,14,20) + c(7,6,0))
sam2[,5:7] <- t(t(sam2[,5:7]) * c(1.5,1.5,1) + c(0,0,0.0))
sam2[,8:10] <- sam2[,8:10] * 1.5
round2 <- pbapply(sam2,1,hist_mat,params=params)
c_r2 <- round2 - c(obs_c[1,],obs_s[1,])
```

I evaluate the results

```
par(mfrow=c(2,3))
plot(sam2[,1],c_r2[1,],ylim=c(-10,10),xlab="other",ylab="sprat difference",
     main="Commercial catches")
abline(h=0,col="red")
plot(sam2[,1],c_r2[2,],ylim=c(-10,10),xlab="other",ylab="mackerel difference",
     main="Commercial catches")
abline(h=0,col="red")
plot(sam2[,1],c_r2[3,],ylim=c(-10,10),xlab="other",ylab="cod difference",
     main="Commercial catches")
abline(h=0,col="red")
plot(sam2[,1],c_r2[4,],ylim=c(-10,10),xlab="other",ylab="sprat difference",
     main="Survey catches")
abline(h=0,col="red")
plot(sam2[,1],c_r2[5,],ylim=c(-10,10),xlab="other",ylab="mackerel difference",
     main="Survey catches")
```

```
abline(h=0,col="red")
plot(sam2[,1],c_r2[6,],ylim=c(-10,10),xlab="other",ylab="cod difference",
     main="Survey catches")
abline(h=0,col="red")
```

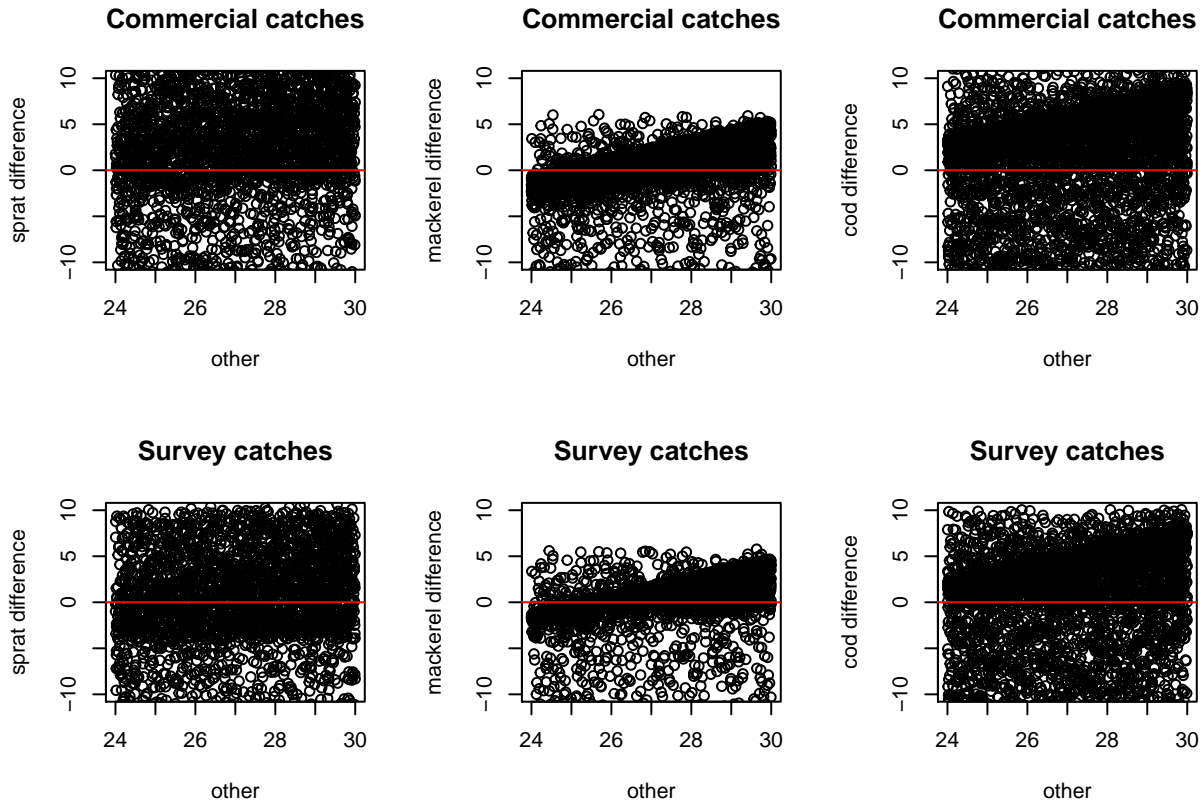

```
par(mfrow=c(2,3))
plot(sam2[,2],c_r2[1,],ylim=c(-10,10),xlab="sprat b",ylab="sprat difference",
     main="Commercial catches")
abline(h=0,col="red")
plot(sam2[,3],c_r2[2,],ylim=c(-10,10),xlab="mackerel b",ylab="mackerel difference",
     main="Commercial catches")
abline(h=0,col="red")
plot(sam2[,4],c_r2[3,],ylim=c(-10,10),xlab="cod b",ylab="cod difference",
     main="Commercial catches")
abline(h=0,col="red")
plot(sam2[,2],c_r2[4,],ylim=c(-10,10),xlab="sprat b",ylab="sprat difference",
     main="Survey catches")
abline(h=0,col="red")
plot(sam2[,3],c_r2[5,],ylim=c(-10,10),xlab="mackerel b",ylab="mackerel difference",
     main="Survey catches")
abline(h=0,col="red")
plot(sam2[,4],c_r2[6,],ylim=c(-10,10),xlab="cod b",ylab="cod difference",
     main="Survey catches")
abline(h=0,col="red")
```

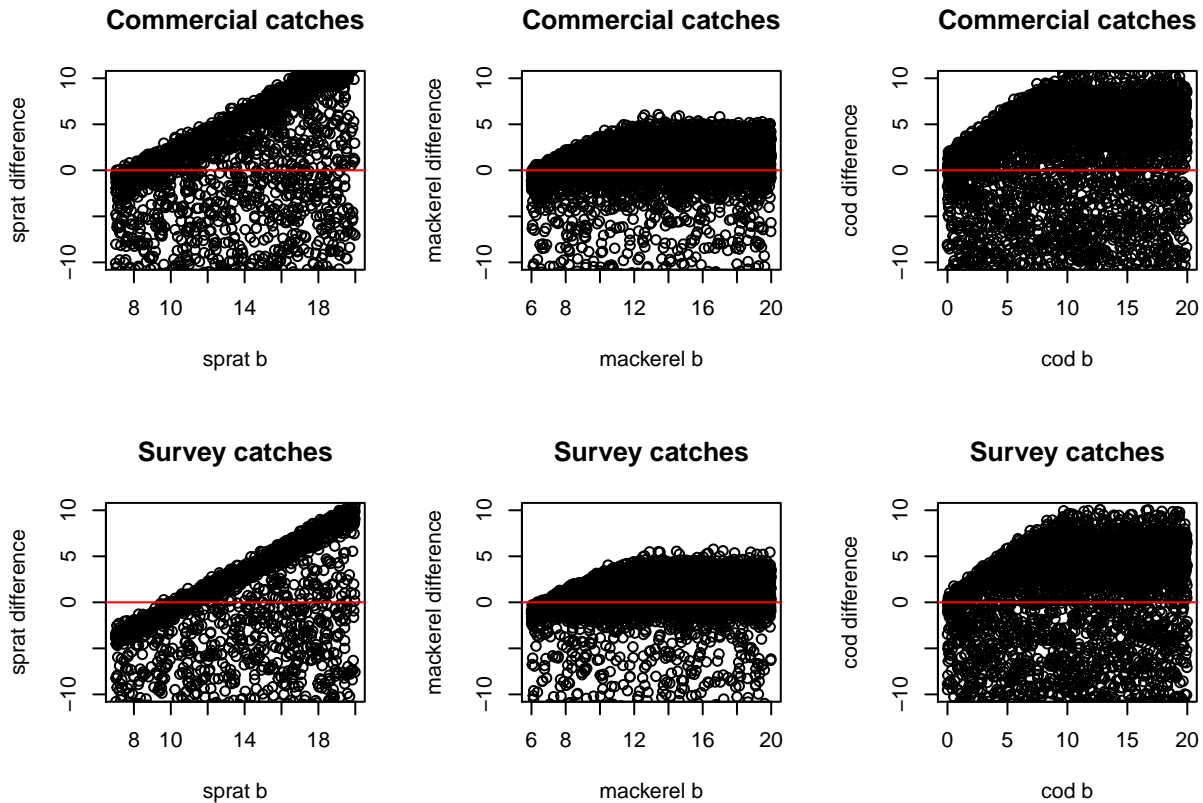

```

par(mfrow=c(2,3))
plot(sam2[,5],c_r2[1,],ylim=c(-10,10),xlab="Spin up F sprat",ylab="sprat difference",
     main="Commercial catches")
abline(h=0,col="red")
plot(sam2[,6],c_r2[2,],ylim=c(-10,10),xlab="Spin up F mackerel",ylab="mackerel difference",
     main="Commercial catches")
abline(h=0,col="red")
plot(sam2[,7],c_r2[3,],ylim=c(-10,10),xlab="Spin up F cod",ylab="cod difference",
     main="Commercial catches")
abline(h=0,col="red")
plot(sam2[,5],c_r2[4,],ylim=c(-10,10),xlab="Spin up F sprat",ylab="sprat difference",
     main="Survey catches")
abline(h=0,col="red")
plot(sam2[,6],c_r2[5,],ylim=c(-10,10),xlab="Spin up F mackerel",ylab="mackerel difference",
     main="Survey catches")
abline(h=0,col="red")
plot(sam2[,7],c_r2[6,],ylim=c(-10,10),xlab="Spin up F cod",ylab="cod difference",
     main="Survey catches")
abline(h=0,col="red")

```

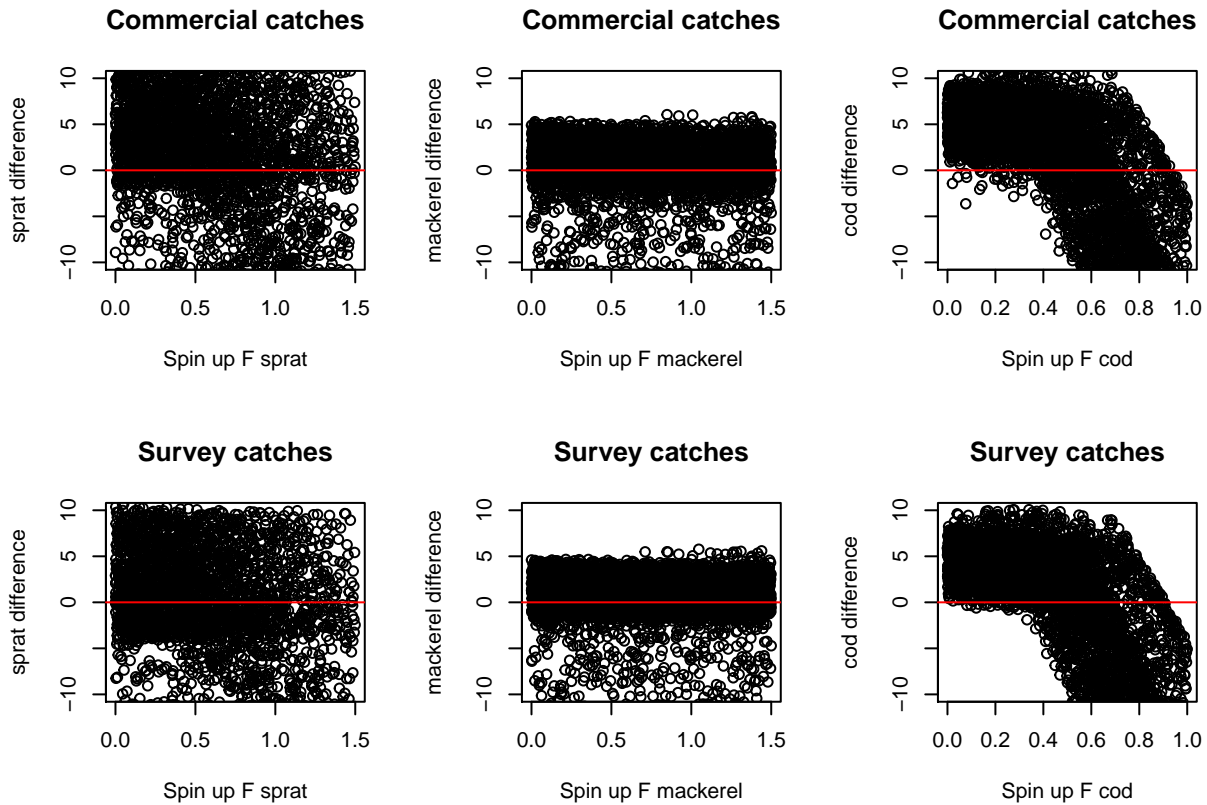

I am happy that I have narrowed down the space and are now happy to setup the MCMC algorithm.

## Markov Chain Monte Carlo

I will first setup the moves. I first setup the likelihood of the full model and the MDA-MCMC algorithm

```
likelihood <- function(obs_c,obs_s,params,model_run,sigma_c,sigma_s,Fs,sur_ef,time=20){
  fish_rate <- cbind(Fs,sur_ef)
  colnames(fish_rate) <- NULL
  catches <- get_CPG(params,model_run,effort=fish_rate)
  com_catches_t <- apply(catches[,1:3,],c(2,3),sum)
  sur_catches <- com_catches <- matrix(0,time,3)
  for (i in 1:time){
    com_catches[i,] <- log(rowSums(com_catches_t[,10 * (i-1) + (1:10)])) - log(1e6)
    sur_catches[i,] <- log(rowSums(catches[,4,10 * (i-1) + (1:10)])) - log(1e6)
  }
  return(rbind(dnorm(t(obs_c),t(com_catches),sigma_c,log=T),
               dnorm(t(obs_s),t(sur_catches),sigma_s,log=T)))
}

get_likelihood<- function(theta,Fs,params,sur_ef,sigma_c,sigma_s,obs_c=obs_c,obs_s=obs_s){
  params@other <- exp(theta[1])
  params@recruit_params[[1]][2] <- exp(theta[2])
  params@recruit_params[[2]][2] <- exp(theta[3])
  params@recruit_params[[3]][2] <- exp(theta[4]);
  tmp <- theta[5:7]
```

```

model_run <- run_LeMans(params, years=100, effort=t(matrix(c(tmp,0),4,100)))
fish_rate <- as.matrix(cbind(Fs,sur_ef))
colnames(fish_rate) <- NULL
model_run_act <- run_LeMans(params, years=20, effort=fish_rate,
                           NO=model_run@N[, ,dim(model_run@N)[3]])

#browser()
like<- likelihood(obs_c,obs_s,params,model_run_act,sigma_c,sigma_s,Fs,sur_ef)
return(list(like=like,model_run=model_run))
}

mda_mcmc <- function(params,model_run,theta,Fs,sur_ef,prop_sdR,prop_sdF,
                    sigma_c,sigma_s,obs_c,obs_s,like){
  prop_ <- parSapply(cl,1:3,mda_mcmc1,params=params,theta=theta,Fs=Fs,
                    sur_ef=sur_ef,prop_sdR=prop_sdR,prop_sdF=prop_sdF,sigma_c=sigma_c,
                    sigma_s=sigma_s,obs_c=obs_c,obs_s=obs_s,like=like)
  thetar <- matrix(rep(c(theta[1],prop_[2,],prop_[3,]),4),4,byrow=T)
  for (i in 2:4){
    thetar[i,c(i,i + 3)] <- c(prop_[c(4,5),i-1])
  }
  like_ <- parRapply(cl,tetar,get_likelihood,Fs=Fs,params=params,sur_ef=sur_ef,
                    sigma_c=sigma_c,sigma_s=sigma_s,obs_c=obs_c,obs_s=obs_s)
  tmp <- lapply(like_[-1],function(x,y){rowSums(x[[1]]-y)},y=like_[[1]][[1]])
  tmp1 <- matrix(unlist(tmp),nrow=3,byrow = T)
  tmp <- c(tmp1[1,1] + tmp1[1,4],tmp1[2,2] + tmp1[2,5],tmp1[3,3] + tmp1[3,6])
  tmp1 <- ifelse(tmp > 0,1,exp(tmp))
  acc_rej<- sum(like_[[1]][[1]]) - sum(like)
  - sum(log(ifelse(prop_[6,]==1,prop_[1,],1-prop_[1,])))
  + sum(log(ifelse(prop_[6,]==1,tmp1,1-tmp1)))
  if (log(runif(1)) < acc_rej){
    print("accept")
    return(list(tetar[1,],like_[[1]][[2]],like_[[1]][[1]]))
  }
  return(list(theta,model_run,like))
}

mda_mcmc1 <- function(i,params,theta,Fs,sur_ef,prop_sdR,prop_sdF,sigma_c,sigma_s,
                    obs_c,obs_s,like){
  theta_ <- rnorm(1,theta[i+1],prop_sdR[i])
  spin_upF_ <- abs(rnorm(1,theta[i+4],prop_sdF[i]))
  params@recruit_params[[1]][2] <- exp(theta[2])
  params@recruit_params[[2]][2] <- exp(theta[3])
  params@recruit_params[[3]][2] <- exp(theta[4]);
  params@recruit_params[[i]][2] <- exp(theta_)
  params@other <- exp(theta[1])
  tmp <- theta[5:7]
  tmp[i] <- spin_upF_
  model_run <- run_LeMans(params, years=100, effort=t(matrix(c(tmp,0),4,100)))
  fish_rate <- as.matrix(cbind(Fs,sur_ef))
  colnames(fish_rate) <- NULL
  model_run_act <- run_LeMans(params, years=20, effort=fish_rate,
                           NO=model_run@N[, ,dim(model_run@N)[3]])
  like_ <- sum(likelihood(obs_c,obs_s,params,model_run_act,
                        sigma_c,sigma_s,Fs,sur_ef)[c(i,i+3),])

```

```

alpha <- exp(min(0, like_ - sum(like[c(i,i+3),])))
if (runif(1) <= alpha){
  return(c(alpha, theta_, spin_upF_, theta[i+1], theta[i+4], 1))
}
return(c(alpha, theta[i+1], theta[i+4], theta_, spin_upF_, 0))
}

```

In this case the likelihood was split into 3:

$$\prod_{t=1}^{20} N(\ln(w_{i,t}) | \ln(c(M_{i,t}(\theta, \phi_{1:20,1:3}))), \sigma_{c,i}^2) N(\ln(z_{i,t}) | \ln(b(M_{i,t}(\theta, \phi_{1:20,1:3}))), \sigma_{s,i}^2),$$

with  $i = 1, 2$  and  $3$ , and the 3 sets of parameters  $\{\theta_2, \theta_5\}$ ,  $\{\theta_3, \theta_6\}$  and  $\{\theta_4, \theta_7\}$  respectively. I setup the Calderhead (2014) move:

```

calderhead_move <- function(params, model_run, theta, Fs, sur_ef, cd_calder_move,
                             sigma_c, sigma_s, obs_c, obs_s, like, M=10){
  theta1 <- as.numeric(theta + t(cd_calder_move) %*% rnorm(7) )
  theta_ <- abs(cbind(theta, theta1 + t(cd_calder_move) %*%
    matrix(rnorm(7 * M), nrow=7, ncol=M) ))
  theta_[1,]<- ifelse(theta_[1,] > 30, 60 - theta_[1,], theta_[1,])
  like_ <- parCapply(cl, theta_, get_likelihood, Fs=Fs, params=params,
    sur_ef=sur_ef, sigma_c=sigma_c, sigma_s=sigma_s,
    obs_c=obs_c, obs_s=obs_s)
  tmp <- unlist(lapply(like_, function(x){sum(x[[1]])}))
  number <- sample(M+1, 1, prob=exp(tmp - max(tmp)))
  print(number)
  return(list(as.numeric(theta_[,number]), like_[[number]][[2]], like_[[number]][[1]]))
}

```

The PDA-MCMC algorithm is setup as follows. First I setup the likelihood and then run through the PDA-MCMC algorithm. In the PDA-MCMC algorithm I only change a few fishing rates at a time, controlled by the change input.

```

log_like <- function(model_run, i, obs_c, obs_s, sigma_c, sigma_s, fishing_rate){
  catches <- get_CPG(params, model_run, effort=fishing_rate)
  com_catches_t <- apply(catches[, 1:3, ], c(2,3), sum)
  com_catches <- log(rowSums(com_catches_t[, (1:10)])) - log(1e6)
  sur_catches <- log(rowSums(catches[, 4, (1:10)])) - log(1e6)
  return(sum(dnorm(obs_c[i,], com_catches, sigma_c, log=T)
    + dnorm(obs_s[i,], sur_catches, sigma_s, log=T)))
}

pda_mcmc <- function(obs_c, obs_s, theta, params, model_run, sigma_c,
                     sigma_s, Fs, sur_ef, llike, sigmasFF, change=1:20){
  params@other <- exp(theta[1])
  params@recruit_params[[1]][2] <- exp(theta[2])
  params@recruit_params[[2]][2] <- exp(theta[3])
  params@recruit_params[[3]][2] <- exp(theta[4])
  tmp <- theta[5:7]
  fish_rate <- cbind(Fs, sur_ef)
  colnames(fish_rate) <- NULL
  Q_0_ <- Q_0 <- M_0 <- model_run
  fish_rate_ <- fish_rate
  alpha <- rep(0)
  alpha1 <- rep(0)
  llike_ <- 0

```

```

hast <- 0
for (i in 1:20){
  if (any(change==i)){
    tmp <- rnorm(3,log(fish_rate[i,1:3]),sigmasFF)
    if (all(exp(tmp) < 2)){
      M_0_ <- run_LeMans(params, years=1,
                        effort=t(c(exp(tmp),fish_rate[i,4])),
                        NO=M_0@N[,dim(M_0@N)[3]])
      ll_p <- log_like(M_0_,i,obs_c,obs_s,sigma_c,sigma_s,
                      t(c(exp(tmp),fish_rate[i,4])))
      Q_0_ <- run_LeMans(params, years=1, effort=t(c(exp(tmp),fish_rate[i,4])),
                        NO=Q_0@N[,dim(Q_0@N)[3]])
      alpha1b <- log_like(Q_0_,i,obs_c,obs_s,sigma_c,sigma_s,
                        t(c(exp(tmp),fish_rate[i,4])))
    }
    else{
      ll_p <- -Inf
      alpha1 <- Inf
      alpha1b <- -Inf
    }
    M_0 <- run_LeMans(params, years=1, effort=t(fish_rate[i,]),
                    NO=M_0@N[,dim(M_0@N)[3]])
    Q_0 <- run_LeMans(params, years=1, effort=t(fish_rate[i,]),
                    NO=Q_0@N[,dim(Q_0@N)[3]])
    ll_r <- log_like(M_0,i,obs_c,obs_s,sigma_c,sigma_s,t(fish_rate[i,]))
    alpha1a <- log_like(Q_0,i,obs_c,obs_s,sigma_c,sigma_s,t(fish_rate[i,]))
    alpha1 <- exp(alpha1a - alpha1b)
    alpha <- min(1,exp(ll_p - ll_r))

    if( runif(1) <= alpha){
      llike_ <- llike_ + ll_p
      M_0 <- M_0_
      fish_rate_[i,] <- c(exp(tmp),fish_rate[i,4])
      hast <- hast + log(min(alpha1,1)) - log(alpha)
    }
    else{
      llike_ <- llike_ + ll_r
      fish_rate_[i,] <- fish_rate[i,]
      hast <- hast + log(1 - min(1/alpha1,1)) - log(1 - alpha)
    }
  }else{
    M_0 <- run_LeMans(params, years=1, effort=t(fish_rate[i,]),
                    NO=M_0@N[,dim(M_0@N)[3]])
    Q_0 <- run_LeMans(params, years=1, effort=t(fish_rate[i,]),
                    NO=Q_0@N[,dim(Q_0@N)[3]])
    llike_ <- llike_ + log_like(M_0,i,obs_c,obs_s,sigma_c,
                              sigma_s,t(fish_rate[i,]))
  }
}
if(log(runif(1)) < (llike_ - llike + hast)){
  print("accept fish_rate")
  return(list(llike=llike_,fish_rate=fish_rate_[1:3]))
}

```

```

else{
  return(list(llike=llike,fish_rate=fish_rate[,1:3]))
}
}

```

I included print statements in the functions so that I could monitor the efficiency of the algorithm. The final updates were the Gibbs steps for the variance parameters.

```

gibbs_move <- function(params,model_run,theta,Fs,sur_ef){
  params@other <- exp(theta[1])
  params@recruit_params[[1]][2] <- exp(theta[2])
  params@recruit_params[[2]][2] <- exp(theta[3])
  params@recruit_params[[3]][2] <- exp(theta[4])
  tmp <- theta[5:7]
  fish_rate <- as.matrix(cbind(Fs,sur_ef))
  colnames(fish_rate) <- NULL
  model_run_act <- run_LeMans(params, years=20, effort=fish_rate,
                             NO=model_run@N[,dim(model_run@N)[3]])
  catches <- get_CPG(params,model_run_act,effort=fish_rate)
  com_catches_t <- apply(catches[,1:3,],c(2,3),sum)
  sur_catches <- com_catches <- matrix(0,20,3)
  for (i in 1:20){
    com_catches[i,] <- log(rowSums(com_catches_t[,10 * (i-1) + (1:10)]))
    - log(1e6)
    sur_catches[i,] <- log(rowSums(catches[,4,10 * (i-1) + (1:10)]))
    - log(1e6)
  }
  sigma_c <- sqrt(1/rgamma(3,shape=10 + 0.1,rate=0.1+
    rowSums((t(obs_c)-t(com_catches))^2)/2))
  sigma_s <- sqrt(1/rgamma(3,shape=10 + 0.1,rate=0.1 +
    rowSums((t(obs_s)-t(sur_catches))^2)/2))
  return(list(sigma_c,sigma_s,rbind(dnorm(t(obs_c),t(com_catches),
    sigma_c,log=T),dnorm(t(obs_s),
    t(sur_catches),sigma_s,log=T))))
}

```

The Caulderhead MCMC algorithm and the MDA-MCMC were run using parallel computing. The PDA-MCMC algorithm was not. LeMans is more computational efficient than mizer and therefore there was no computational saving by doing this algorithm in parallel.

For a wider discussion about tuning MCMC see Bédard (2019).

I chose initial parameters to start the MCMC. I got these from the history matching.

```

theta <- c(24, 10,6,0, 0.5,0.5,0.5)
Fs <- matrix(runif(20 * 3 ,0,1.5),20,3)
sigma_s <- c(0.5,0.5,0.5)
sigma_c <- c(0.5,0.5,0.5)

```

I set the tuning parameters for the MCMC algorithm, tuned from a pilot run of the MCMC. For the MDA-MCMC algorithm I set the standard deviation of the recruitment parameters to be 0.2 and the **spinupF** to be 0.1. In this algorithm one can be bold with the moves of the parameters. The standard deviation on the natural log scale for the fish rates is 0.2. I tuned this by visually checking that the traceplots were sufficiently uncorrelated.

```

prop_sdR <- c(0.2,0.2,0.2)
prop_sdF <- c(0.1,0.1,0.1)

```

```
sigmasFF <- 0.2
```

I also set the `cd_calder_move` move covariance matrix. This was also tuned by visually checking that the traceplots were sufficiently uncorrelated. I set it to be

```
cd_calder_move
```

```
##           [,1]      [,2]      [,3]      [,4]      [,5]
## [1,] 0.3181287 -0.16571338 -0.10798335 -0.058822985 0.007216805
## [2,] 0.0000000 0.06771038 0.05815456 0.025367897 0.008722411
## [3,] 0.0000000 0.00000000 0.04012165 0.004443627 -0.017053754
## [4,] 0.0000000 0.00000000 0.00000000 0.023845481 -0.011498798
## [5,] 0.0000000 0.00000000 0.00000000 0.000000000 0.128449775
## [6,] 0.0000000 0.00000000 0.00000000 0.000000000 0.000000000
## [7,] 0.0000000 0.00000000 0.00000000 0.000000000 0.000000000
##           [,6]      [,7]
## [1,] -0.035365868 0.0007653306
## [2,] 0.010598455 0.0013499564
## [3,] 0.005688382 0.0020397175
## [4,] -0.003254364 0.0103733712
## [5,] 0.067451182 0.0061164841
## [6,] 0.109961896 0.0086195768
## [7,] 0.000000000 0.0256809963
```

`cd_calder_move` is the transpose of the Cholesky decomposition of the covariance matrix used when proposing new `theta` values. I setup variables for saving the parameters.

```
library(abind)
thetas <- theta
Fss <- array(Fs,dim=c(20,3,1))
sigmas_s <- sigma_s
sigmas_c <- sigma_c
```

and then calculate the likelihood and model after the spinup period for the current parameter settings.

```
tmp <- get_likelihood(theta,Fs,params,sur_ef,sigma_c,sigma_s,obs_c=obs_c,obs_s=obs_s)
like <- tmp[[1]]; model_run <- tmp[[2]]
```

To get the fishing rates in the ballpark and speeding up the burn-in period of the algorithm I run a version of the PDA-MCMC algorithm, that does not deal with the Hasting ratio.

```
pda_mcmc_spin_up <- function(obs_c,obs_s,theta,params,model_run,sigma_c,
                             sigma_s,Fs,sur_ef,llike,sigmasFF,change=1:20){
  params@other <- exp(theta[1])
  params@recruit_params[[1]][2] <- exp(theta[2])
  params@recruit_params[[2]][2] <- exp(theta[3])
  params@recruit_params[[3]][2] <- exp(theta[4])
  tmp <- theta[5:7]
  fish_rate <- cbind(Fs,sur_ef)
  colnames(fish_rate) <- NULL
  Q_0_ <- Q_0 <- M_0 <- model_run
  fish_rate_ <- fish_rate
  alpha <- rep(0,20)
  alpha1 <- rep(0,20)
  llike_ <- 0
  hast <- 0
  for (i in 1:20){
```

```

if (any(change==i)){
  tmp <- rnorm(3,log(fish_rate[i,1:3]),sigmasFF)
  if (all(exp(tmp) < 2)){
    M_0_ <- run_LeMans(params, years=1, effort=t(c(exp(tmp),fish_rate[i,4])),
                      NO=M_0@N[,dim(M_0@N)[3]])
    ll_p <- log_like(M_0_,i,obs_c,obs_s,sigma_c,sigma_s,
                    t(c(exp(tmp),fish_rate_[i,4])))
  }
  else{
    ll_p <- -Inf
  }
  M_0 <- run_LeMans(params, years=1, effort=t(fish_rate[i,]),
                  NO=M_0@N[,dim(M_0@N)[3]])
  ll_r <- log_like(M_0,i,obs_c,obs_s,sigma_c,sigma_s,
                  t(fish_rate[i,]))
  alpha <- min(1,exp(ll_p - ll_r))
  if( runif(1) <= alpha){
    llike_ <- llike_ + ll_p
    M_0 <- M_0_
    fish_rate_[i,] <- c(exp(tmp),fish_rate[i,4])
  }
  else{
    llike_ <- llike_ + ll_r
    fish_rate_[i,] <- fish_rate[i,]
  }
}
}
else{
  M_0 <- run_LeMans(params, years=1, effort=t(fish_rate[i,]),
                  NO=M_0@N[,dim(M_0@N)[3]])
  llike_ <- llike_ + log_like(M_0,i,obs_c,obs_s,sigma_c,
                              sigma_s,t(fish_rate[i,]))
}
}
}
if(log(runif(1)) < (llike_ - llike)){
  print(paste("accept fish_rate",change))
  return(list(llike=llike_,fish_rate=fish_rate_[,1:3]))
}
else{
  return(list(llike=llike,fish_rate=fish_rate[,1:3]))
}
}

for(ii in 1:1000){
  test <- pda_mcmc_spin_up(obs_c,obs_s,theta,params,model_run,
                          sigma_c,sigma_s,Fs,sur_ef,llike=sum(like),
                          sigmasFF=sigmasFF,change=which(sample(c(0,1),
                                                                20,replace=T,prob=c(0.8,0.2))==1))

  like <- test[[1]]; Fs <- test[[2]]
}

```

I then calculate the likelihood again and save it because in this code the `pda_mcmc` function, as written here, does not give the likelihood in the correct way.

```

tmp <- get_likelihood(theta,Fs,params,sur_ef,sigma_c,sigma_s,obs_c=obs_c,obs_s=obs_s)
like <- tmp[[1]]; model_run <- tmp[[2]]

```

```
likes <- sum(like)
```

I setup the clusters and say that the MCMC will run for 20000 iterations.

```
N <- 2e4
library(parallel)
cl <- makeCluster(10)
clusterExport(cl=cl, c("get_likelihood", "run_LeMans", "likelihood", "get_CPG"))
```

I then run the MCMC algorithm. One iteration of the MCMC will update the parameters according to the MDA-MCMC algorithm; then it will do the PDA-MCMC algorithm 10 times, randomly choosing whether or not update  $\phi_{t,1:3}$  at each  $t$  with probability 0.7; then it will run the caulderheadparallel MCMC with 9 proposals and finally the variance parameters will be updated using the Gibbs steps. I collect the parameters, print the iteration number and every 1000 iterations I look at the traceplot of **theta**.

```
ii <- 1
while(ii < N){
  ## mda-mcmc
  test <- mda_mcmc(params,model_run,theta,Fs,sur_ef,prop_sdR,
                  prop_sdF,sigma_c,sigma_s,obs_c,obs_s,like)
  theta <- test[[1]]; model_run <- test[[2]]; like <- test[[3]]

  ## pda-mcmc
  for(kk in 1:10){
    test <- pda_mcmc(obs_c,obs_s,theta,params,model_run,sigma_c,
                    sigma_s,Fs,sur_ef,llike=sum(like),sigmasFF=sigmasFF,
                    change=which(sample(c(0,1),20,replace=T,prob=c(0.3,0.7))==1))
    like <- test[[1]]; Fs <- test[[2]]
  }

  ## calderhead
  test <- calderhead_move(params,model_run,theta,Fs,sur_ef,cd_calder_move,
                        sigma_c,sigma_s,obs_c,obs_s,like, M=9)
  theta <- test[[1]]; model_run <- test[[2]]; like <- test[[3]]

  ## gibbs move
  test <- gibbs_move(params,model_run,theta,Fs,sur_ef)
  sigma_c <- test[[1]]; sigma_s <- test[[2]]; like <- test[[3]]

  ## collecting
  thetas <- rbind(thetas,theta)
  Fss <- abind(Fss,Fs)
  sigmas_c <- rbind(sigmas_c,sigma_c)
  sigmas_s <- rbind(sigmas_s,sigma_s)
  likes <- c(likes,sum(like))
  if ((ii / 1000) == floor(ii / 1000)){
    plot.ts(thetas)
  }
  ii <- ii + 1
  print(ii)
}
```

I examine the traceplots for the fishing rates

```
plot.ts(t(Fss[1:10,1,]))
```

**t(Fss[1:10, 1, ])**

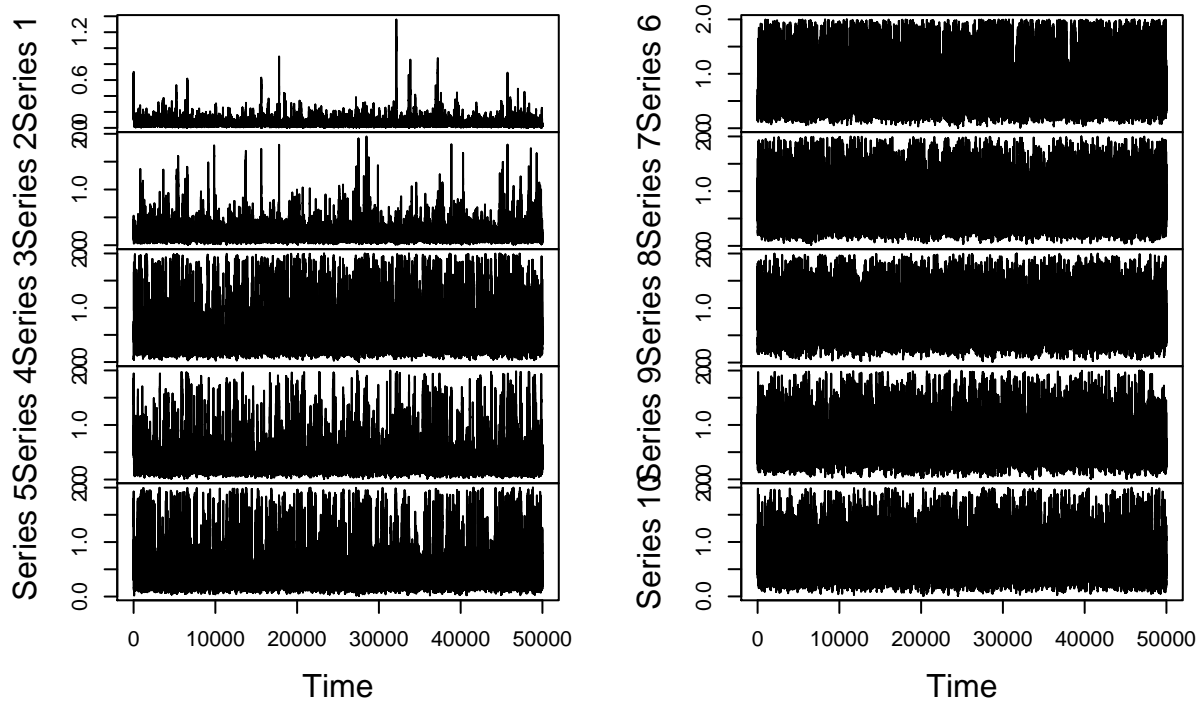

```
plot.ts(t(Fss[1:10,2,]))
```

**t(Fss[1:10, 2, ])**

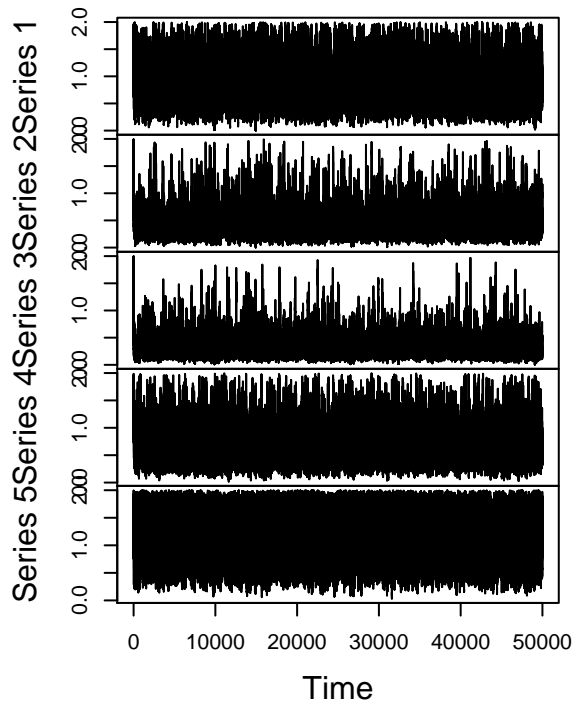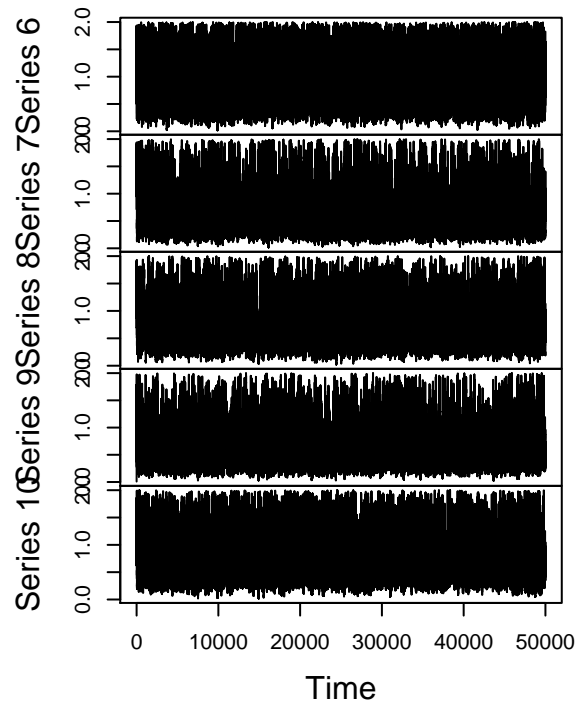

```
plot.ts(t(Fss[1:10,3,]))
```

**t(Fss[1:10, 3, ])**

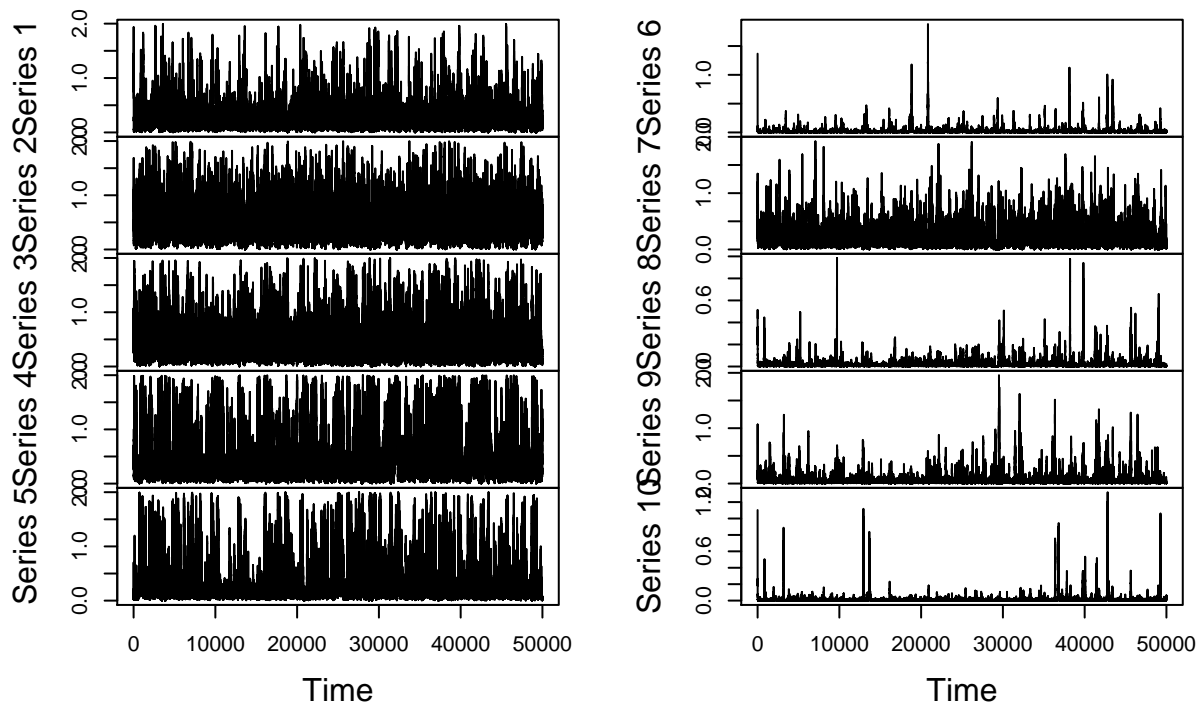

and for the static parameters

```
plot.ts(thetas)
```

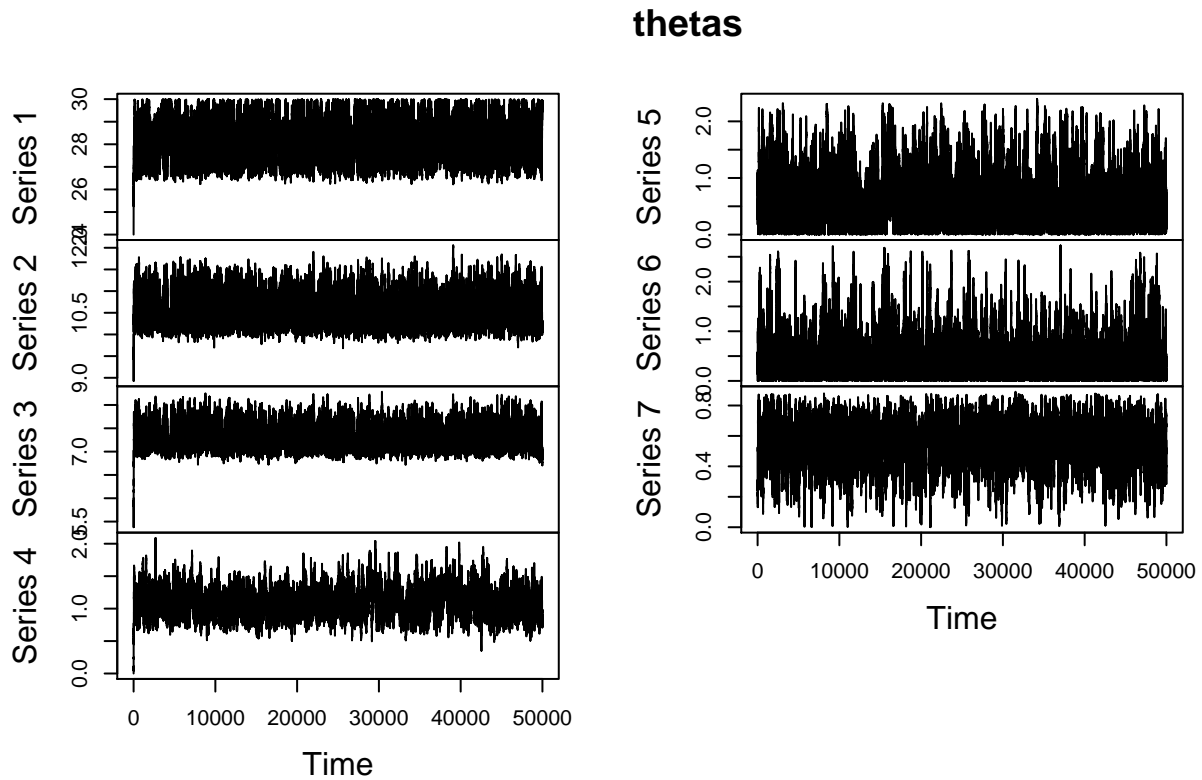

## Results

I discard the first 1000 iterations as burn up. I examine the posterior distribution of the fishing rates,  $\phi_{1:20,1:3}$ . The solid line black line is the median posterior distribution and the dotted lines are the 10th and 90th percentiles. The grey line is the truth.

```
par(mfrow=c(3,1))
par(mar=c(2,2,2,0))
par(oma=c(2.1,2.1,0,0))
tmp<-apply(Fss[,1,-(1:1000)],1,quantile,probs=c(0.1,0.5,0.9))
plot(c(1,20),c(0,2),type="n",main="Sprat",xlab="",ylab="")
lines(1:20,tmp[2,])
lines(1:20,tmp[1,],lty=2)
lines(1:20,tmp[3,],lty=2)
lines(1:20,fish_rate[,1],col="grey")
###
tmp<-apply(Fss[,2,-(1:1000)],1,quantile,probs=c(0.05,0.5,0.95))
plot(c(1,20),c(0,2),type="n",main="Mackerel",xlab="",ylab="")
lines(1:20,tmp[2,])
lines(1:20,tmp[1,],lty=2)
lines(1:20,tmp[3,],lty=2)
lines(1:20,fish_rate[,2],col="grey")
###
tmp<-apply(Fss[,3,-(1:1000)],1,quantile,probs=c(0.05,0.5,0.95))
plot(c(1,20),c(0,2),type="n",main="Cod",xlab="",ylab="")
```

```

lines(1:20,tmp[2,])
lines(1:20,tmp[1,],lty=2)
lines(1:20,tmp[3,],lty=2)
lines(1:20,fish_rate[,3],col="grey")
mtext("Year",side=1,outer = T,line=1)
mtext(expression(phi["1:20,1:3"]),side=2,outer = T,line=1)

```

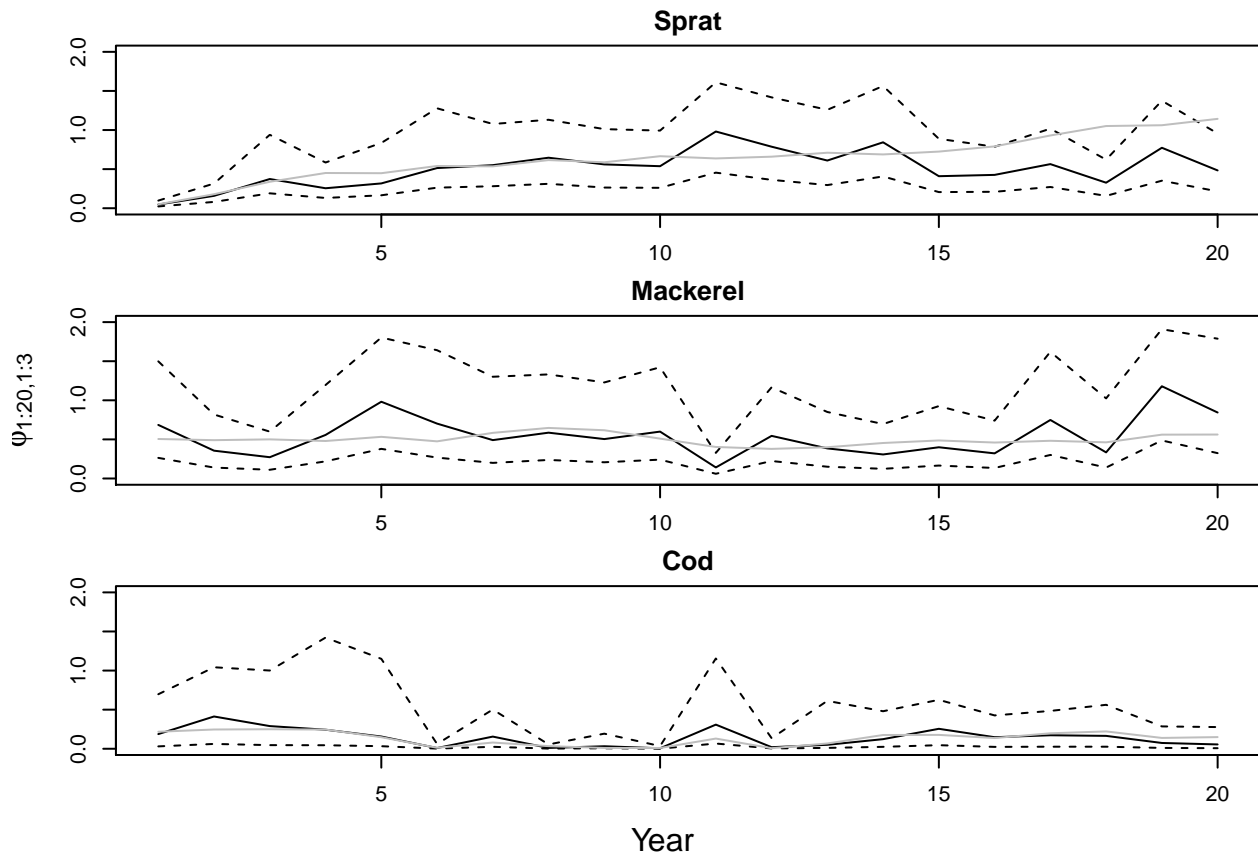

I examine the posterior of the static parameters,  $\theta$ .  $\theta_1$  is below with the truth being the grey line.

```

par(mfrow=c(1,1))
plot(density(thetas[-(1:1000),1]),main="other",xlab=expression(theta[1]))
abline(v=27,col="grey")

```

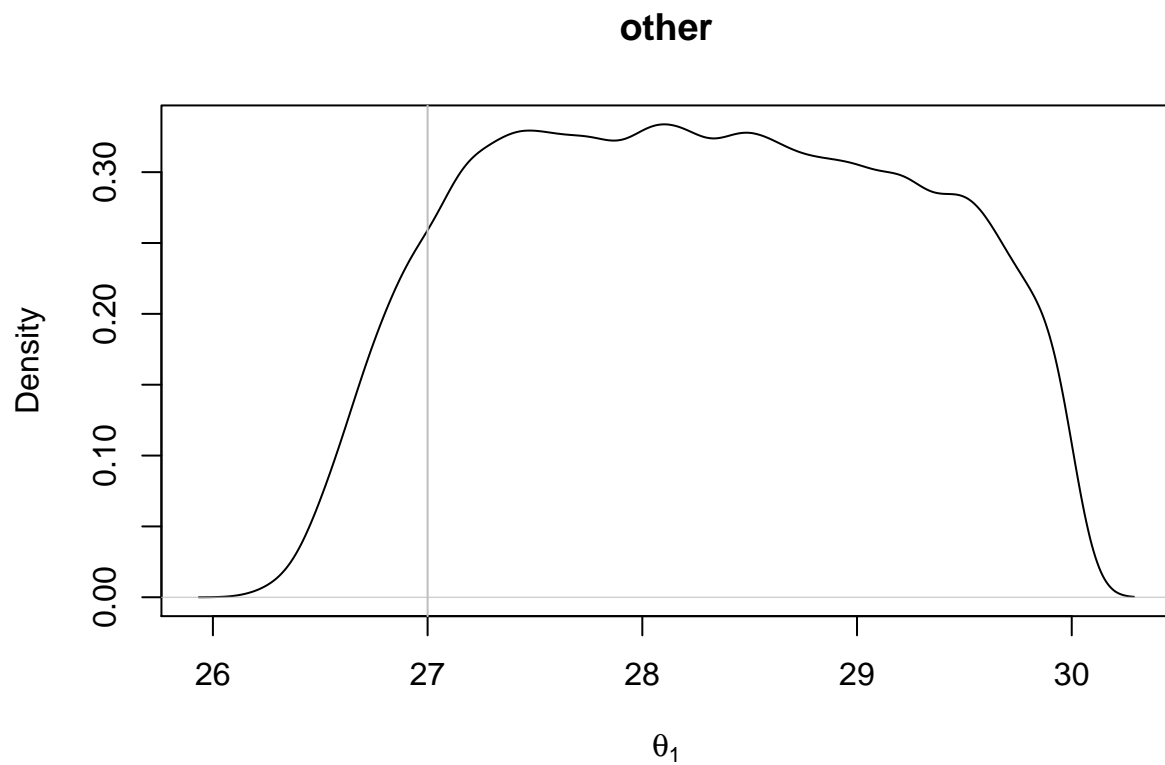

The recruitment and spin up Fs are for Sprat

```
par(mfrow=c(1,2))
plot(density(thetas[-(1:1000),2]),main="",xlab=expression(theta[2]))
abline(v=11,col="grey")
plot(density(thetas[-(1:1000),5]),main="",xlab=expression(theta[5]))
abline(v=0.1,col="grey")
```

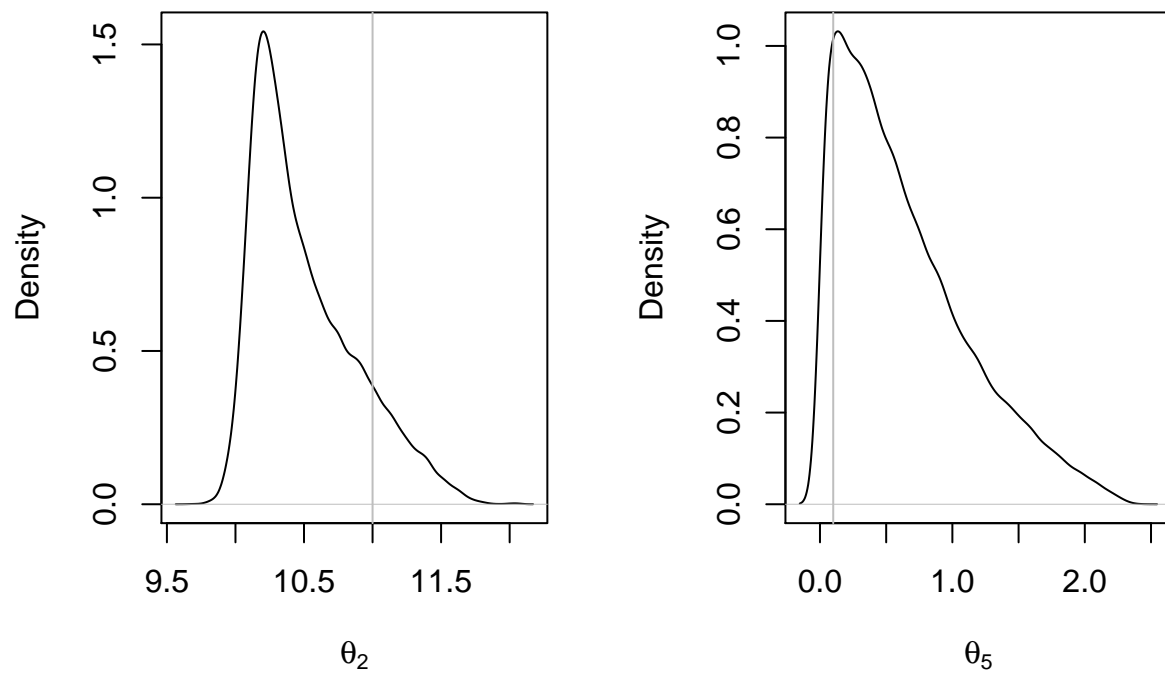

for mackerel

```
par(mfrow=c(1,2))
plot(density(thetas[-(1:1000),3]),main="",xlab=expression(theta[3]))
abline(v=7.5,col="grey")
plot(density(thetas[-(1:1000),6]),main="",xlab=expression(theta[6]))
abline(v=0.3,col="grey")
```

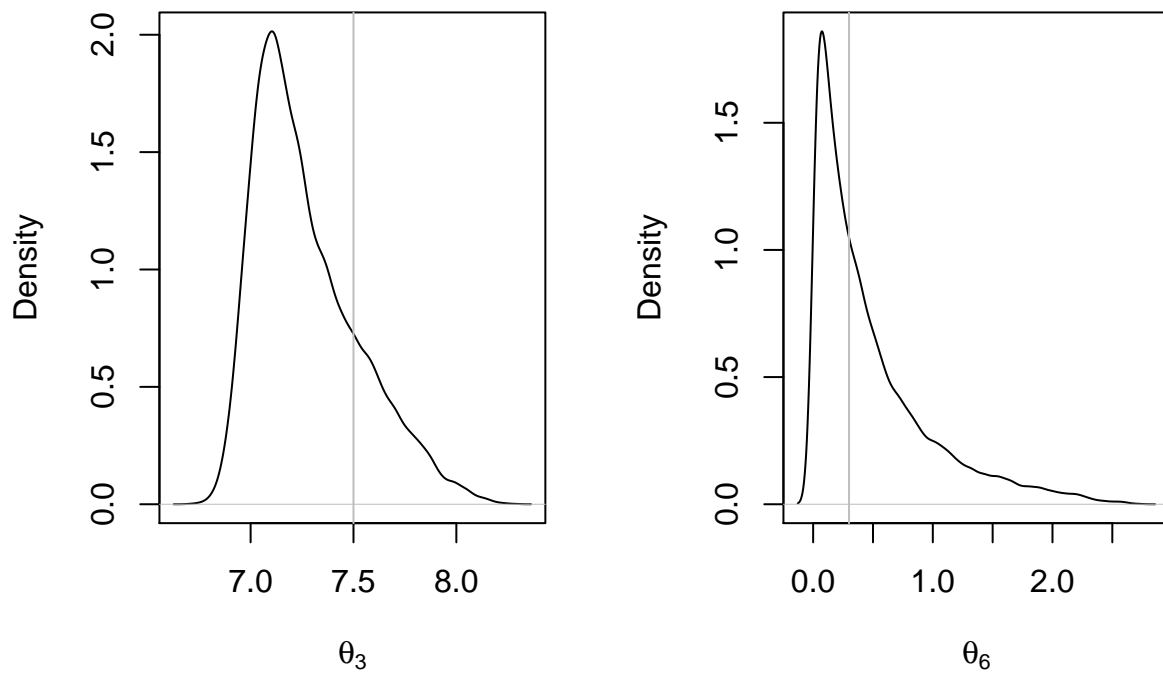

and for cod

```
par(mfrow=c(1,2))
plot(density(thetas[-(1:1000),4]),main="",xlab=expression(theta[4]))
abline(v=1,col="grey")
plot(density(thetas[-(1:1000),7]),main="",xlab=expression(theta[7]))
abline(v=0.6,col="grey")
```

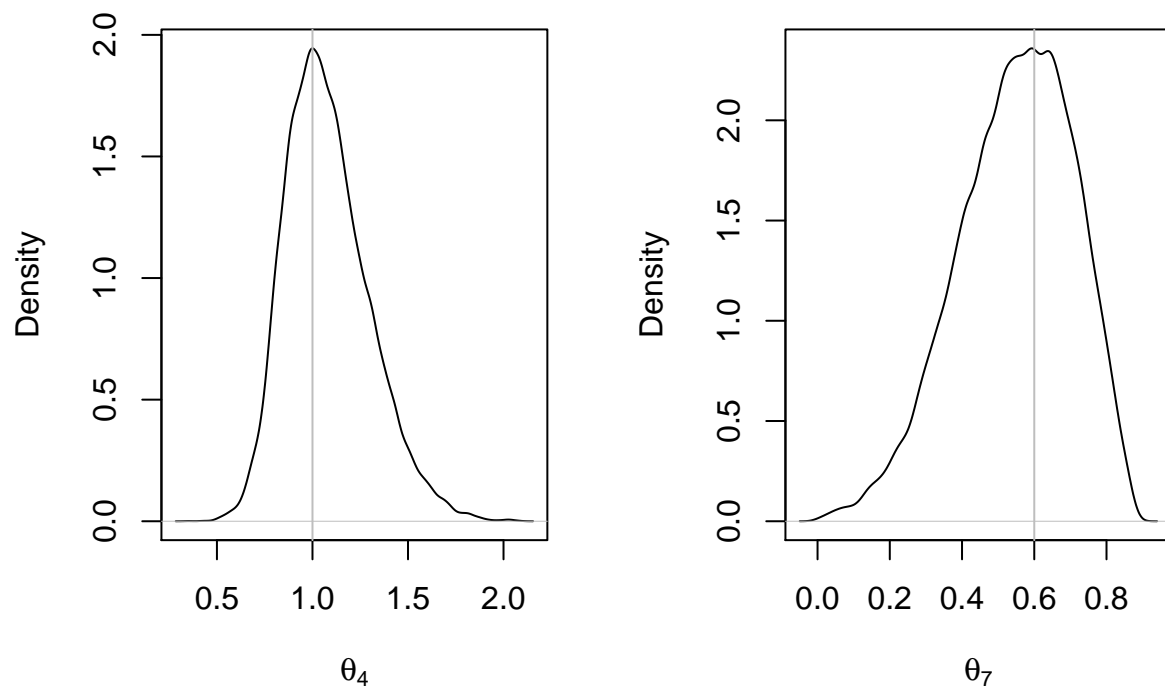

The variance parameters for sprat

```
par(mfrow=c(1,2))
plot(density(sigmasc[-(1:1000),1]),main="",xlab=expression(sigma["c",1]))
abline(v=0.38,col="grey")
plot(density(sigmass[-(1:1000),1]),main="",xlab=expression(sigma["s",1]))
abline(v=0.6,col="grey")
```

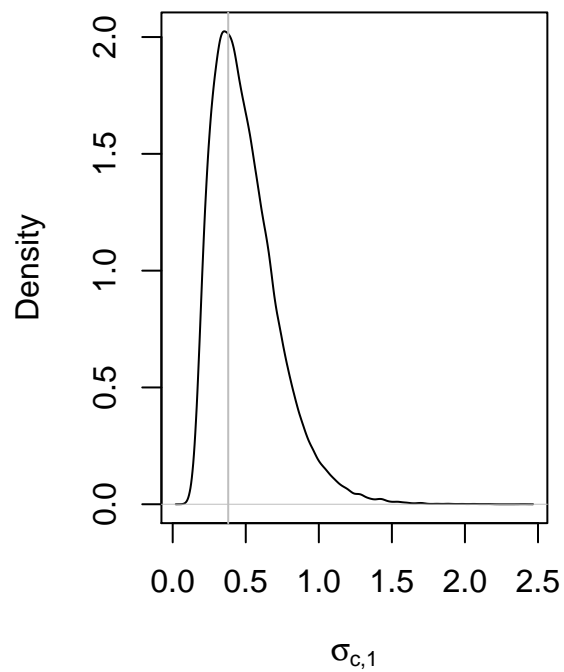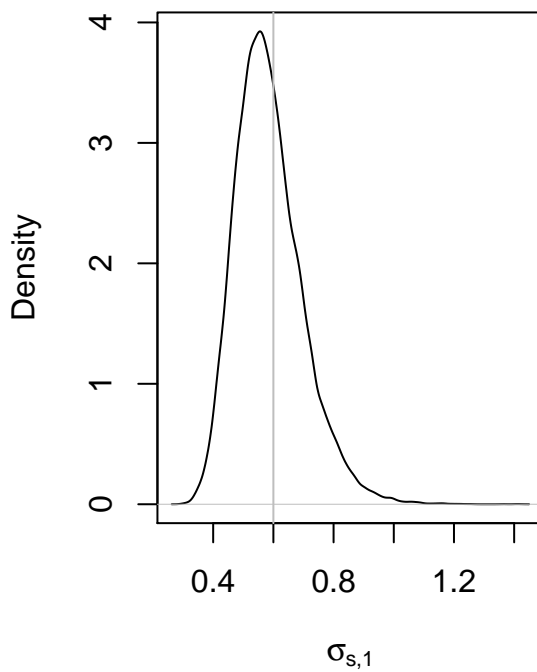

for mackerel

```
par(mfrow=c(1,2))
plot(density(sigmatas_c[-(1:1000),2]),main="",xlab=expression(sigma["c",2]))
abline(v=0.44,col="grey")
plot(density(sigmatas_s[-(1:1000),2]),main="",xlab=expression(sigma["s",2]))
abline(v=0.7,col="grey")
```

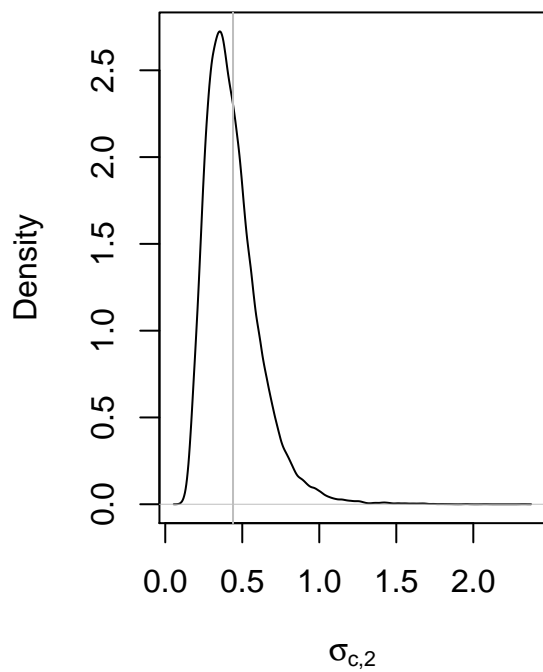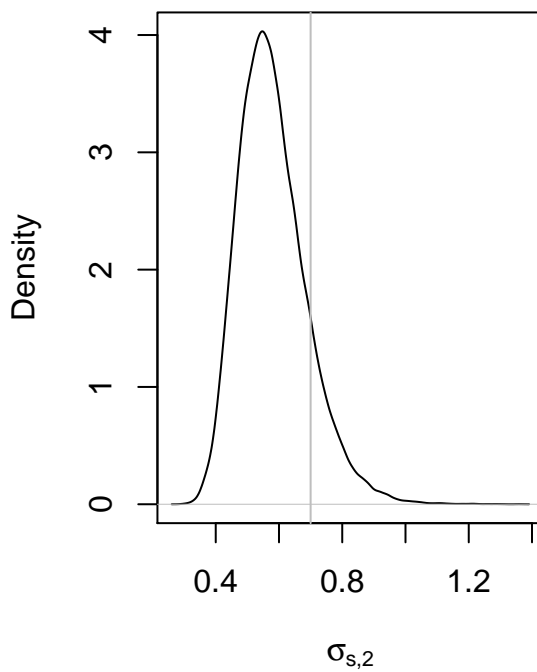

and cod

```
par(mfrow=c(1,2))
plot(density(sigmatas_c[-(1:1000),3]),main="",xlab=expression(sigma["c",3]))
abline(v=0.5,col="grey")
plot(density(sigmatas_s[-(1:1000),3]),main="",xlab=expression(sigma["s",3]))
abline(v=0.6,col="grey")
```

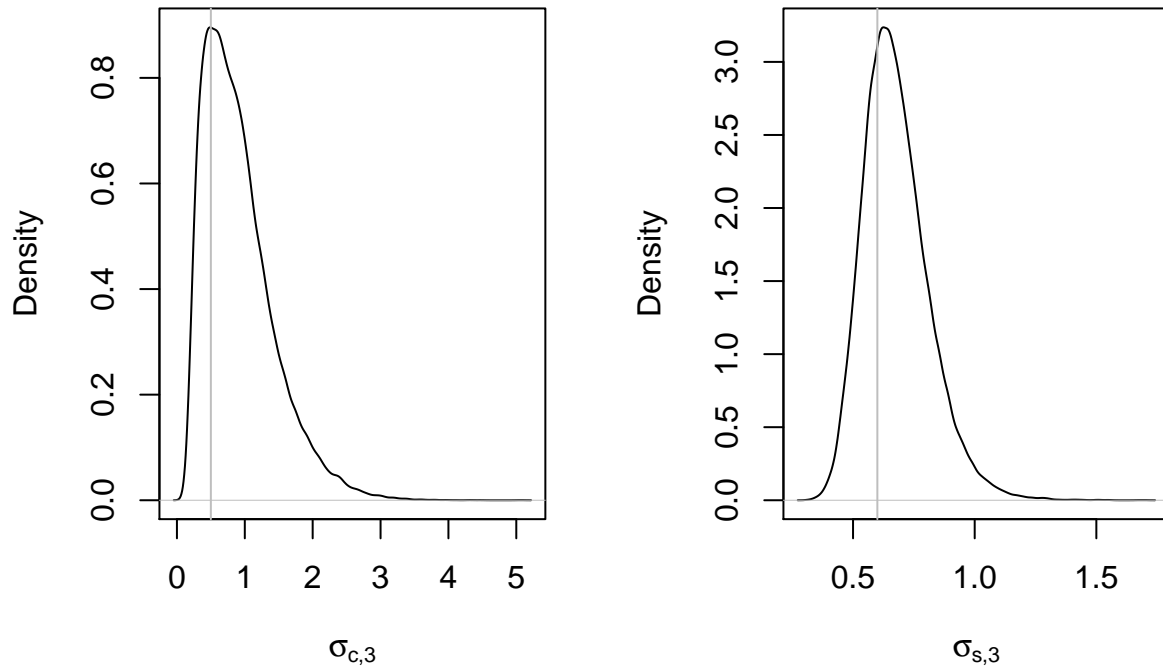

Bédard, Mylène. 2019. “Hierarchical Models and Tuning of Random Walk Metropolis Algorithms.” *Journal of Probability and Statistics* 2019 (August): 8740426. <https://doi.org/10.1155/2019/8740426>.

Calderhead, Ben. 2014. “A General Construction for Parallelizing Metropolis-Hastings Algorithms.” *Proceedings of the National Academy of Sciences* 111 (49): 17408–13. <https://doi.org/10.1073/pnas.1408184111>.

Sobol’, I.M. 1967. “On the Distribution of Points in a Cube and the Approximate Evaluation of Integrals.” *USSR Computational Mathematics and Mathematical Physics* 7 (4): 86–112. [https://doi.org/https://doi.org/10.1016/0041-5553\(67\)90144-9](https://doi.org/https://doi.org/10.1016/0041-5553(67)90144-9).

Spence, Hayley J. AND Ball, Michael A. AND Bannister. 2020. “LeMaRns: A Length-Based Multi-Species Analysis by Numerical Simulation in R.” *PLOS ONE* 15 (2): 1–12. <https://doi.org/10.1371/journal.pone.0227767>.

Thorpe, Robert B., Will J. F. Le Quesne, Fay Luxford, Jeremy S. Collie, and Simon Jennings. 2015. “Evaluation and Management Implications of Uncertainty in a Multispecies Size-Structured Model of Population and Community Responses to Fishing.” *Methods in Ecology and Evolution* 6 (1): 49–58. <https://doi.org/10.1111/2041-210X.12292>.

Walker, Nicola D., David L. Maxwell, Will J. F. Le Quesne, and Simon Jennings. 2017. “Estimating Efficiency of Survey and Commercial Trawl Gears from Comparisons of Catch-Ratios.” *ICES Journal of Marine Science* 74 (5): 1448–57. <https://doi.org/10.1093/icesjms/fsw250>.
